# Supplementary material for: Computational timeline reconstruction of the stories surrounding Trump: Story turbulence, narrative control, and collective chronopathy
Source: arXiv:2008.07301 ancillary file (2022-09-30)

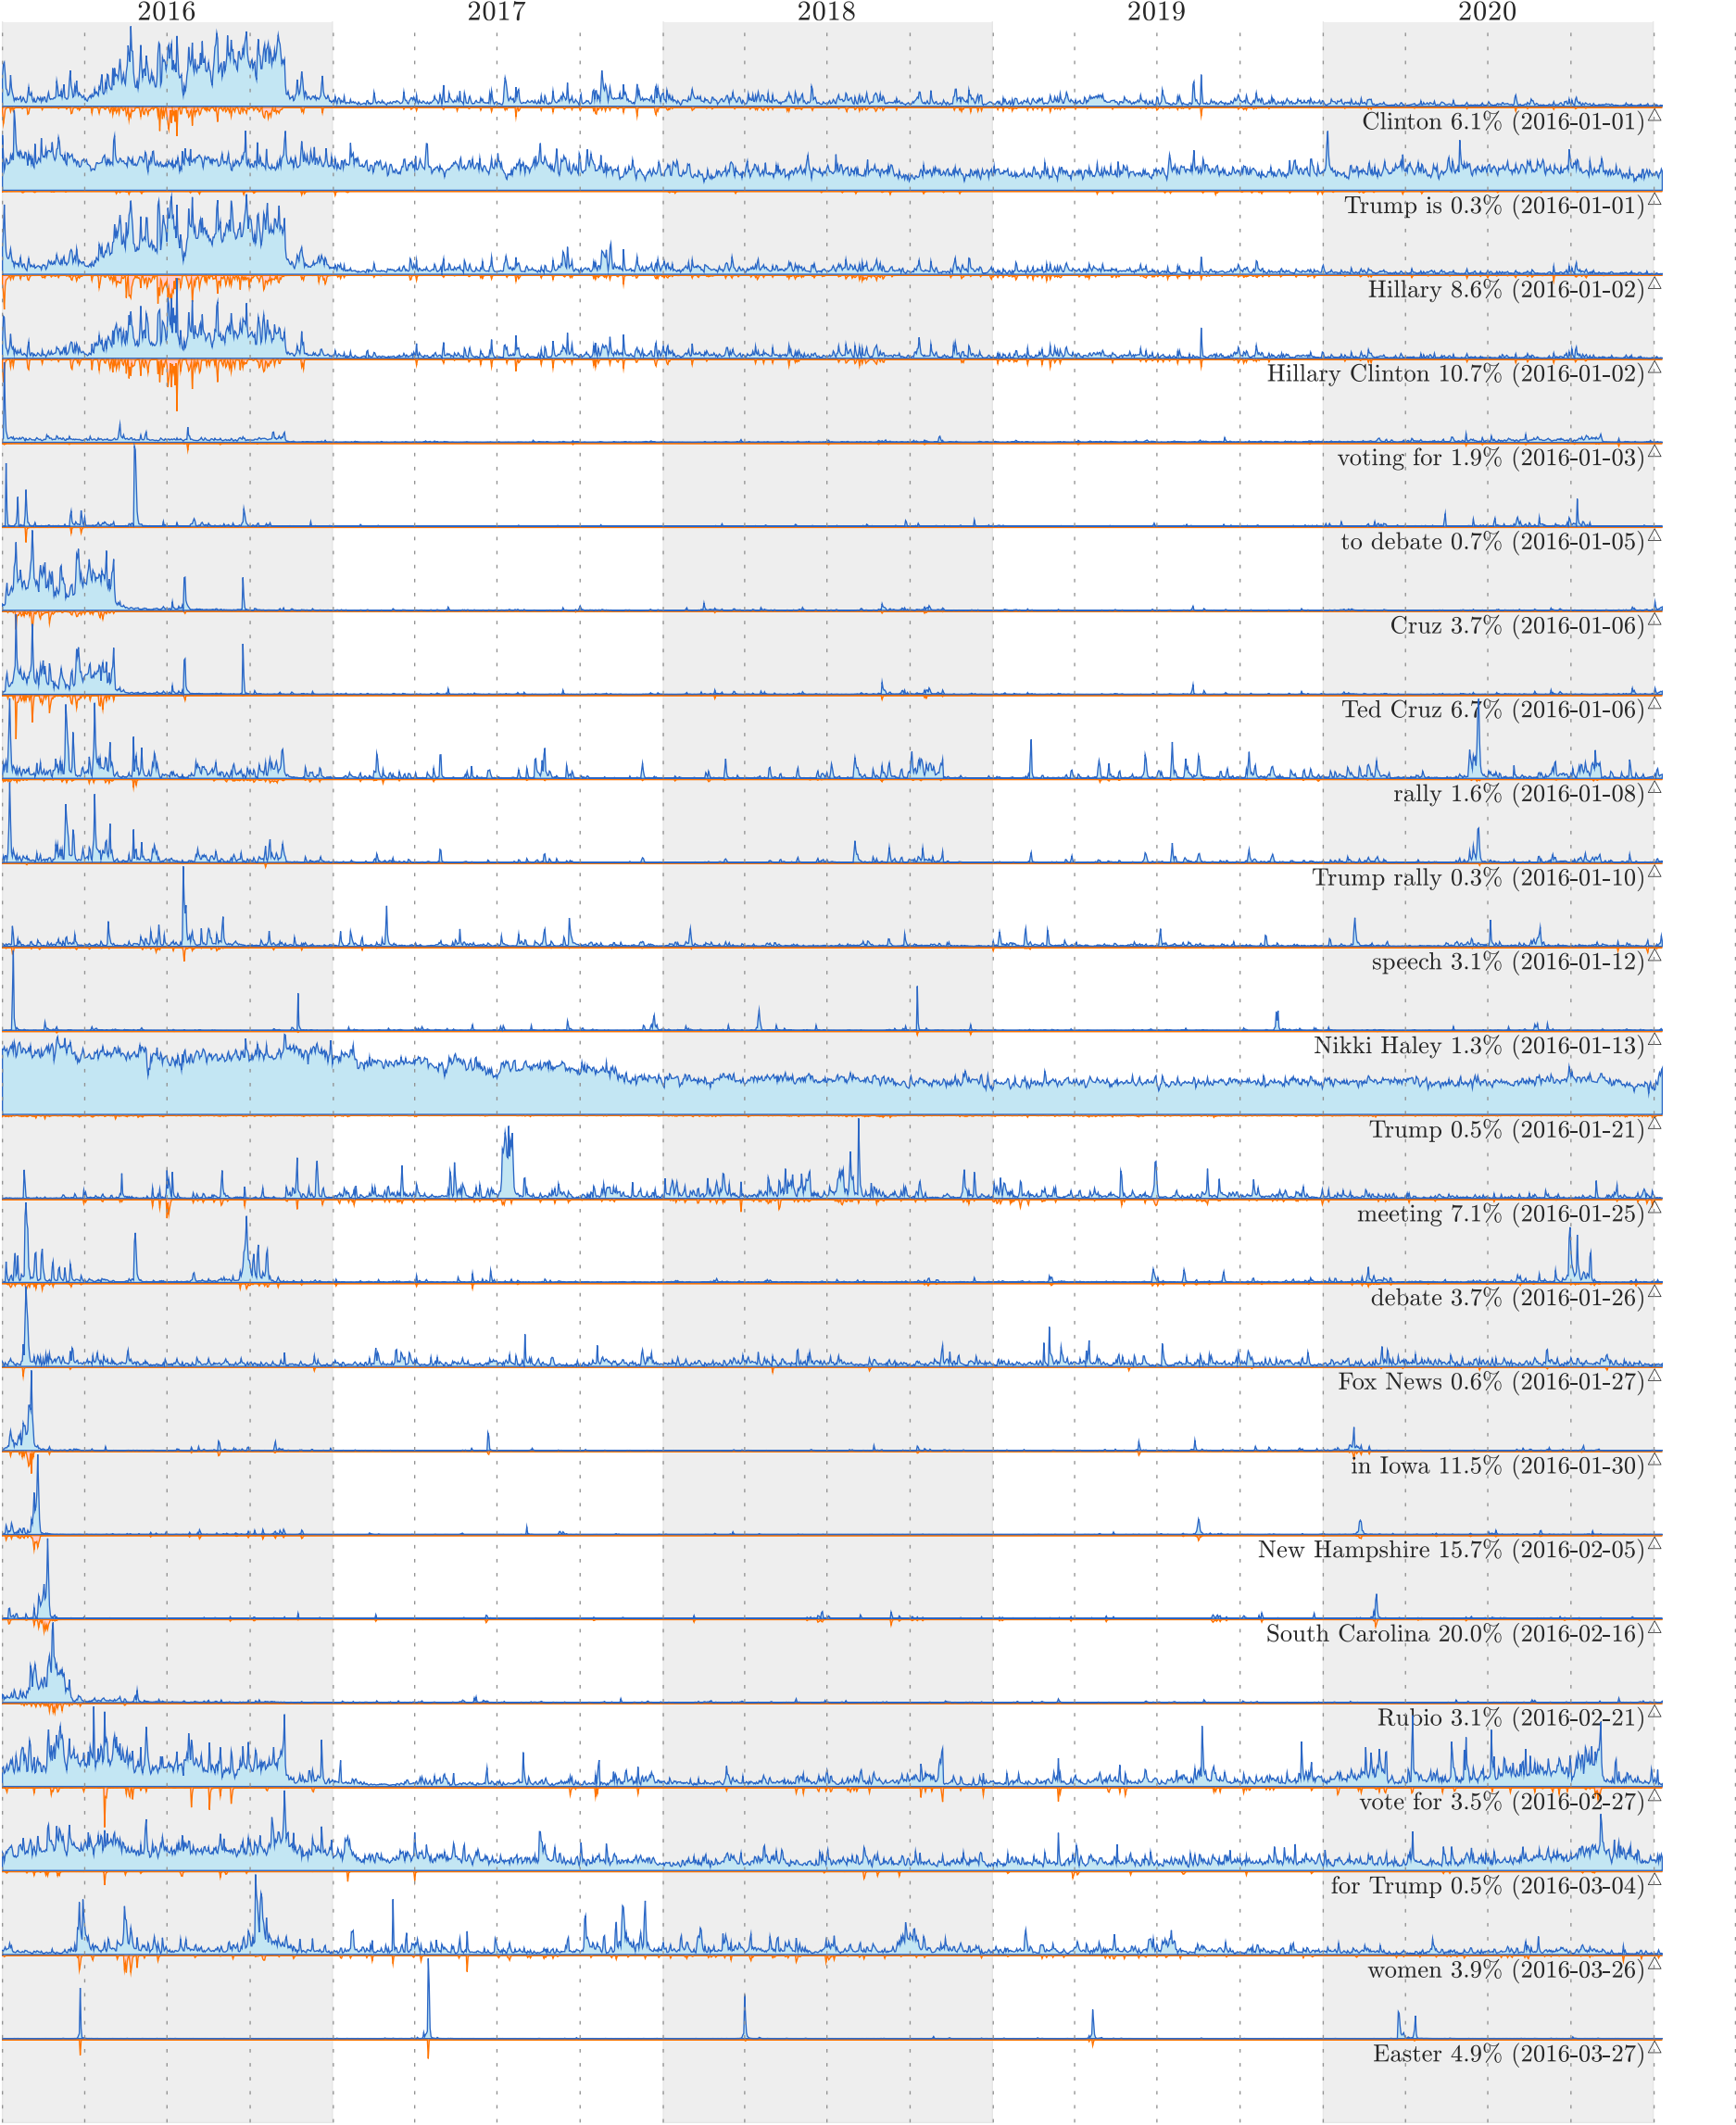

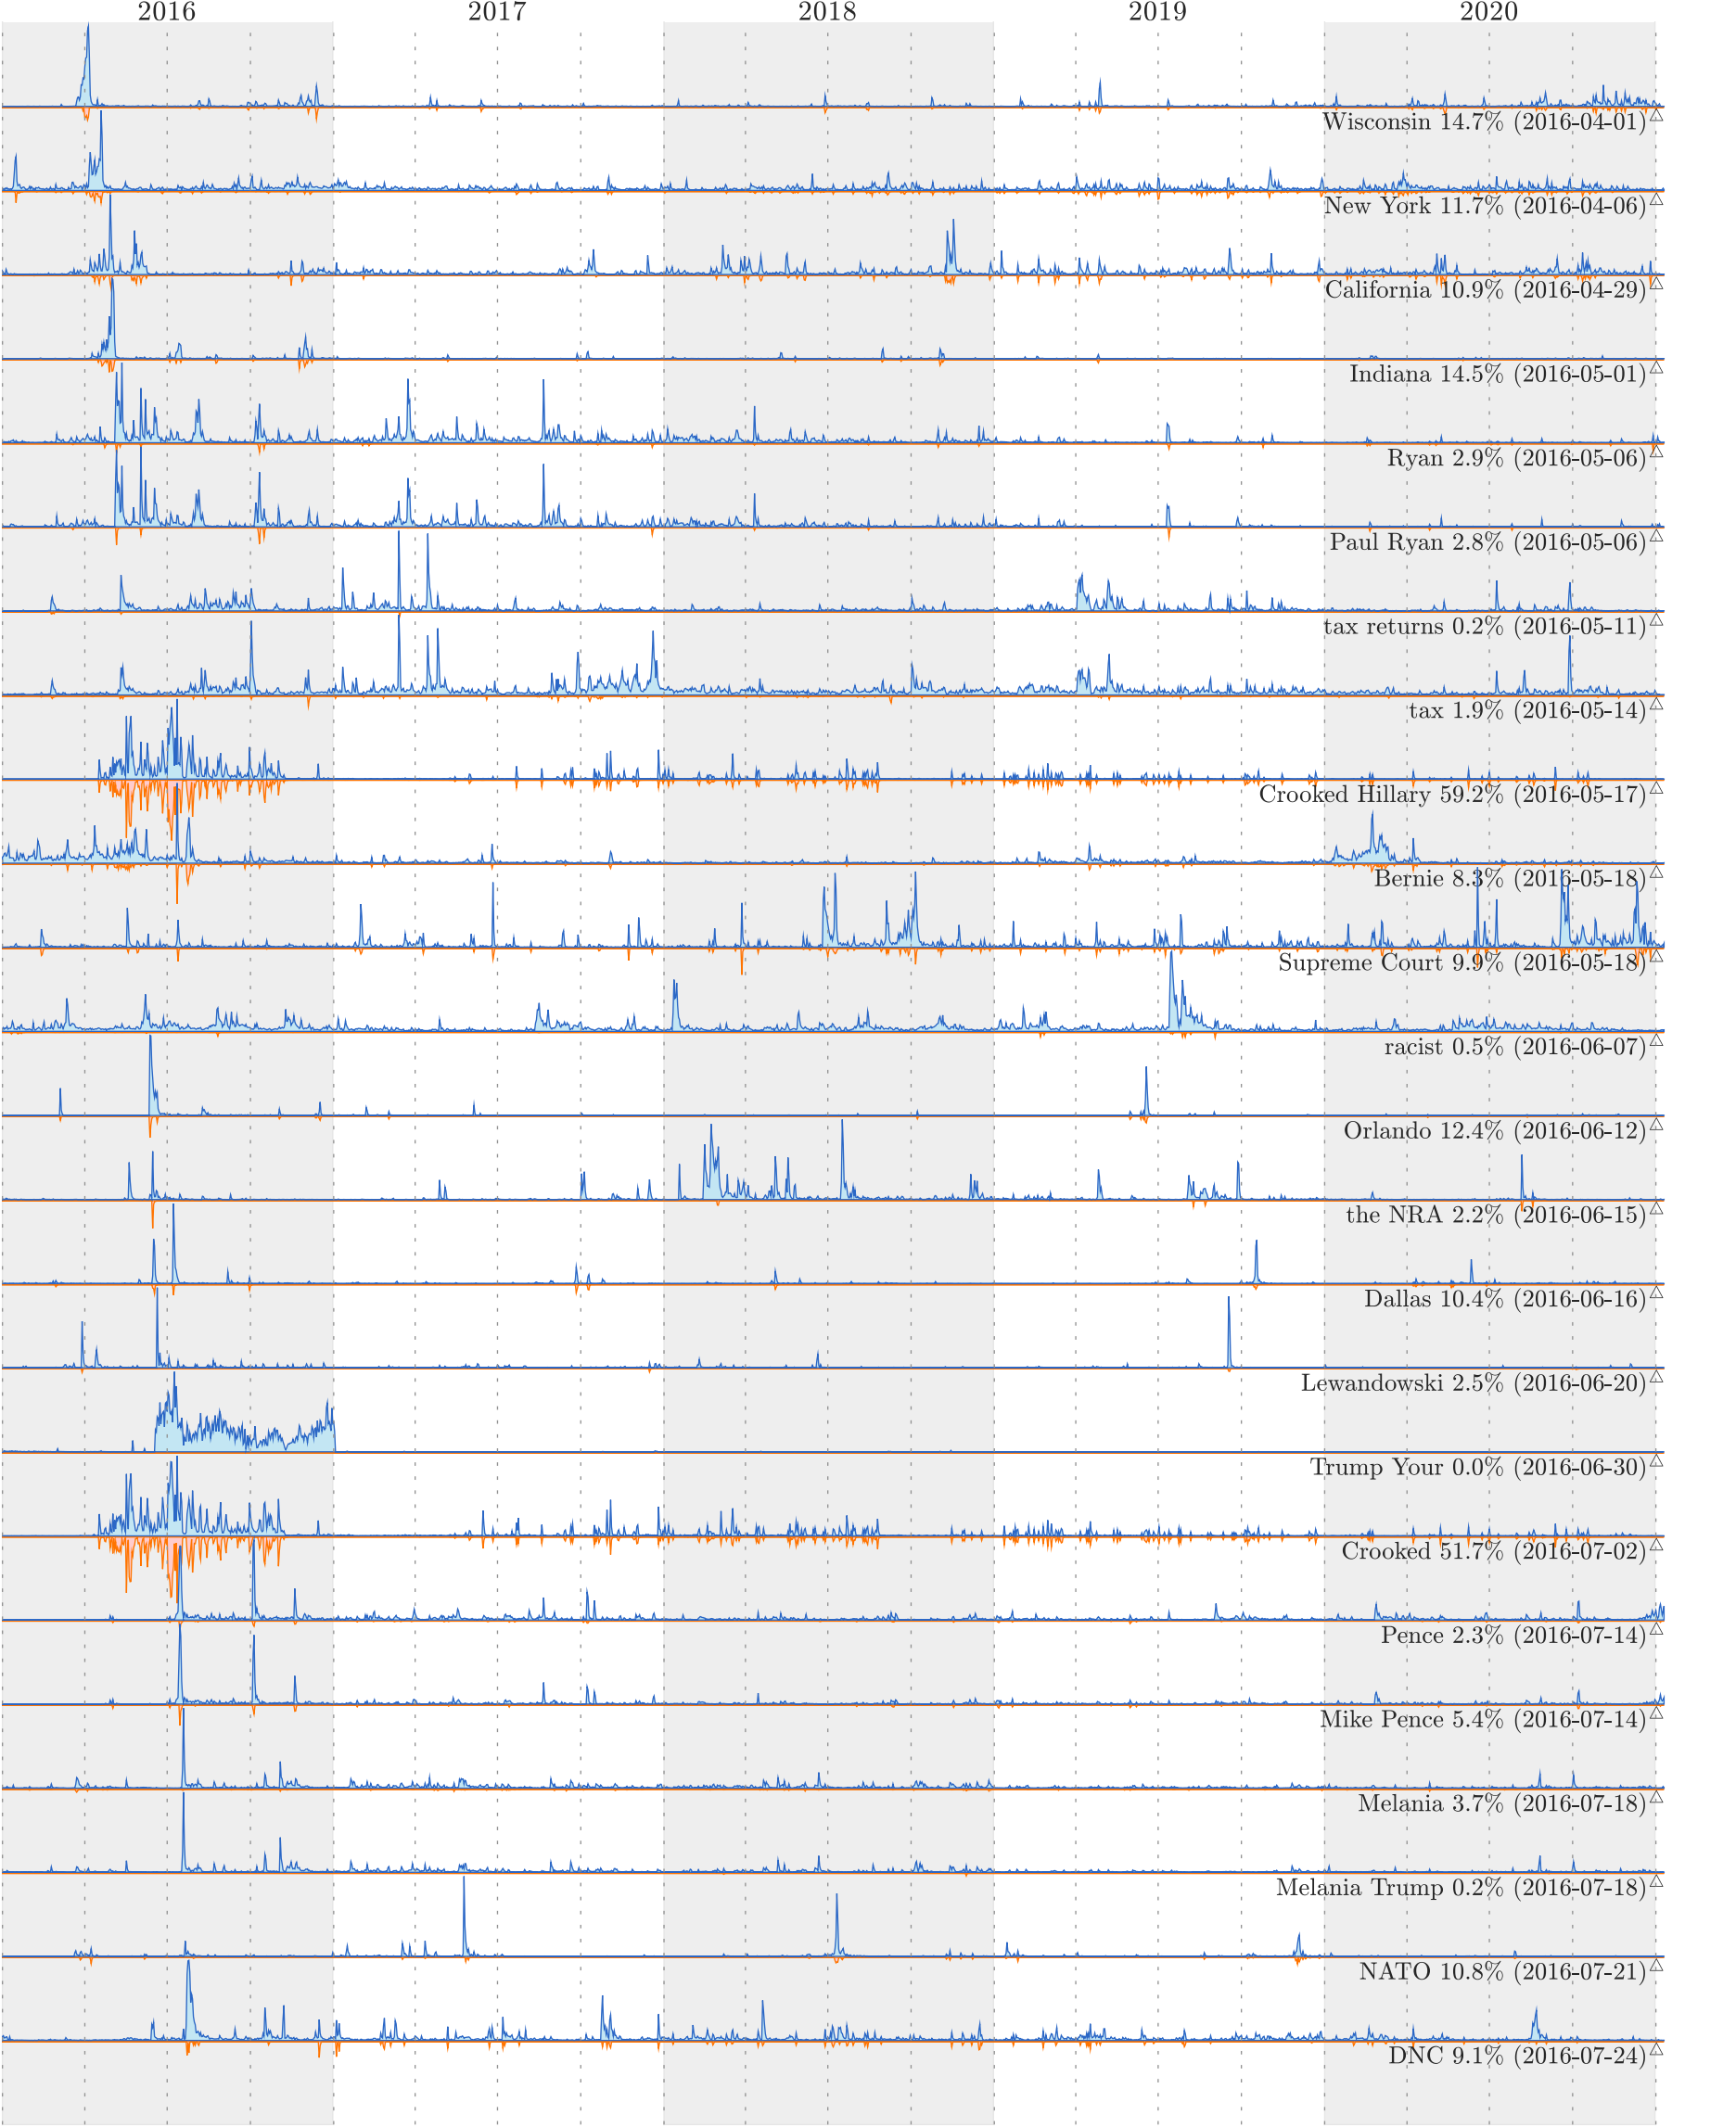

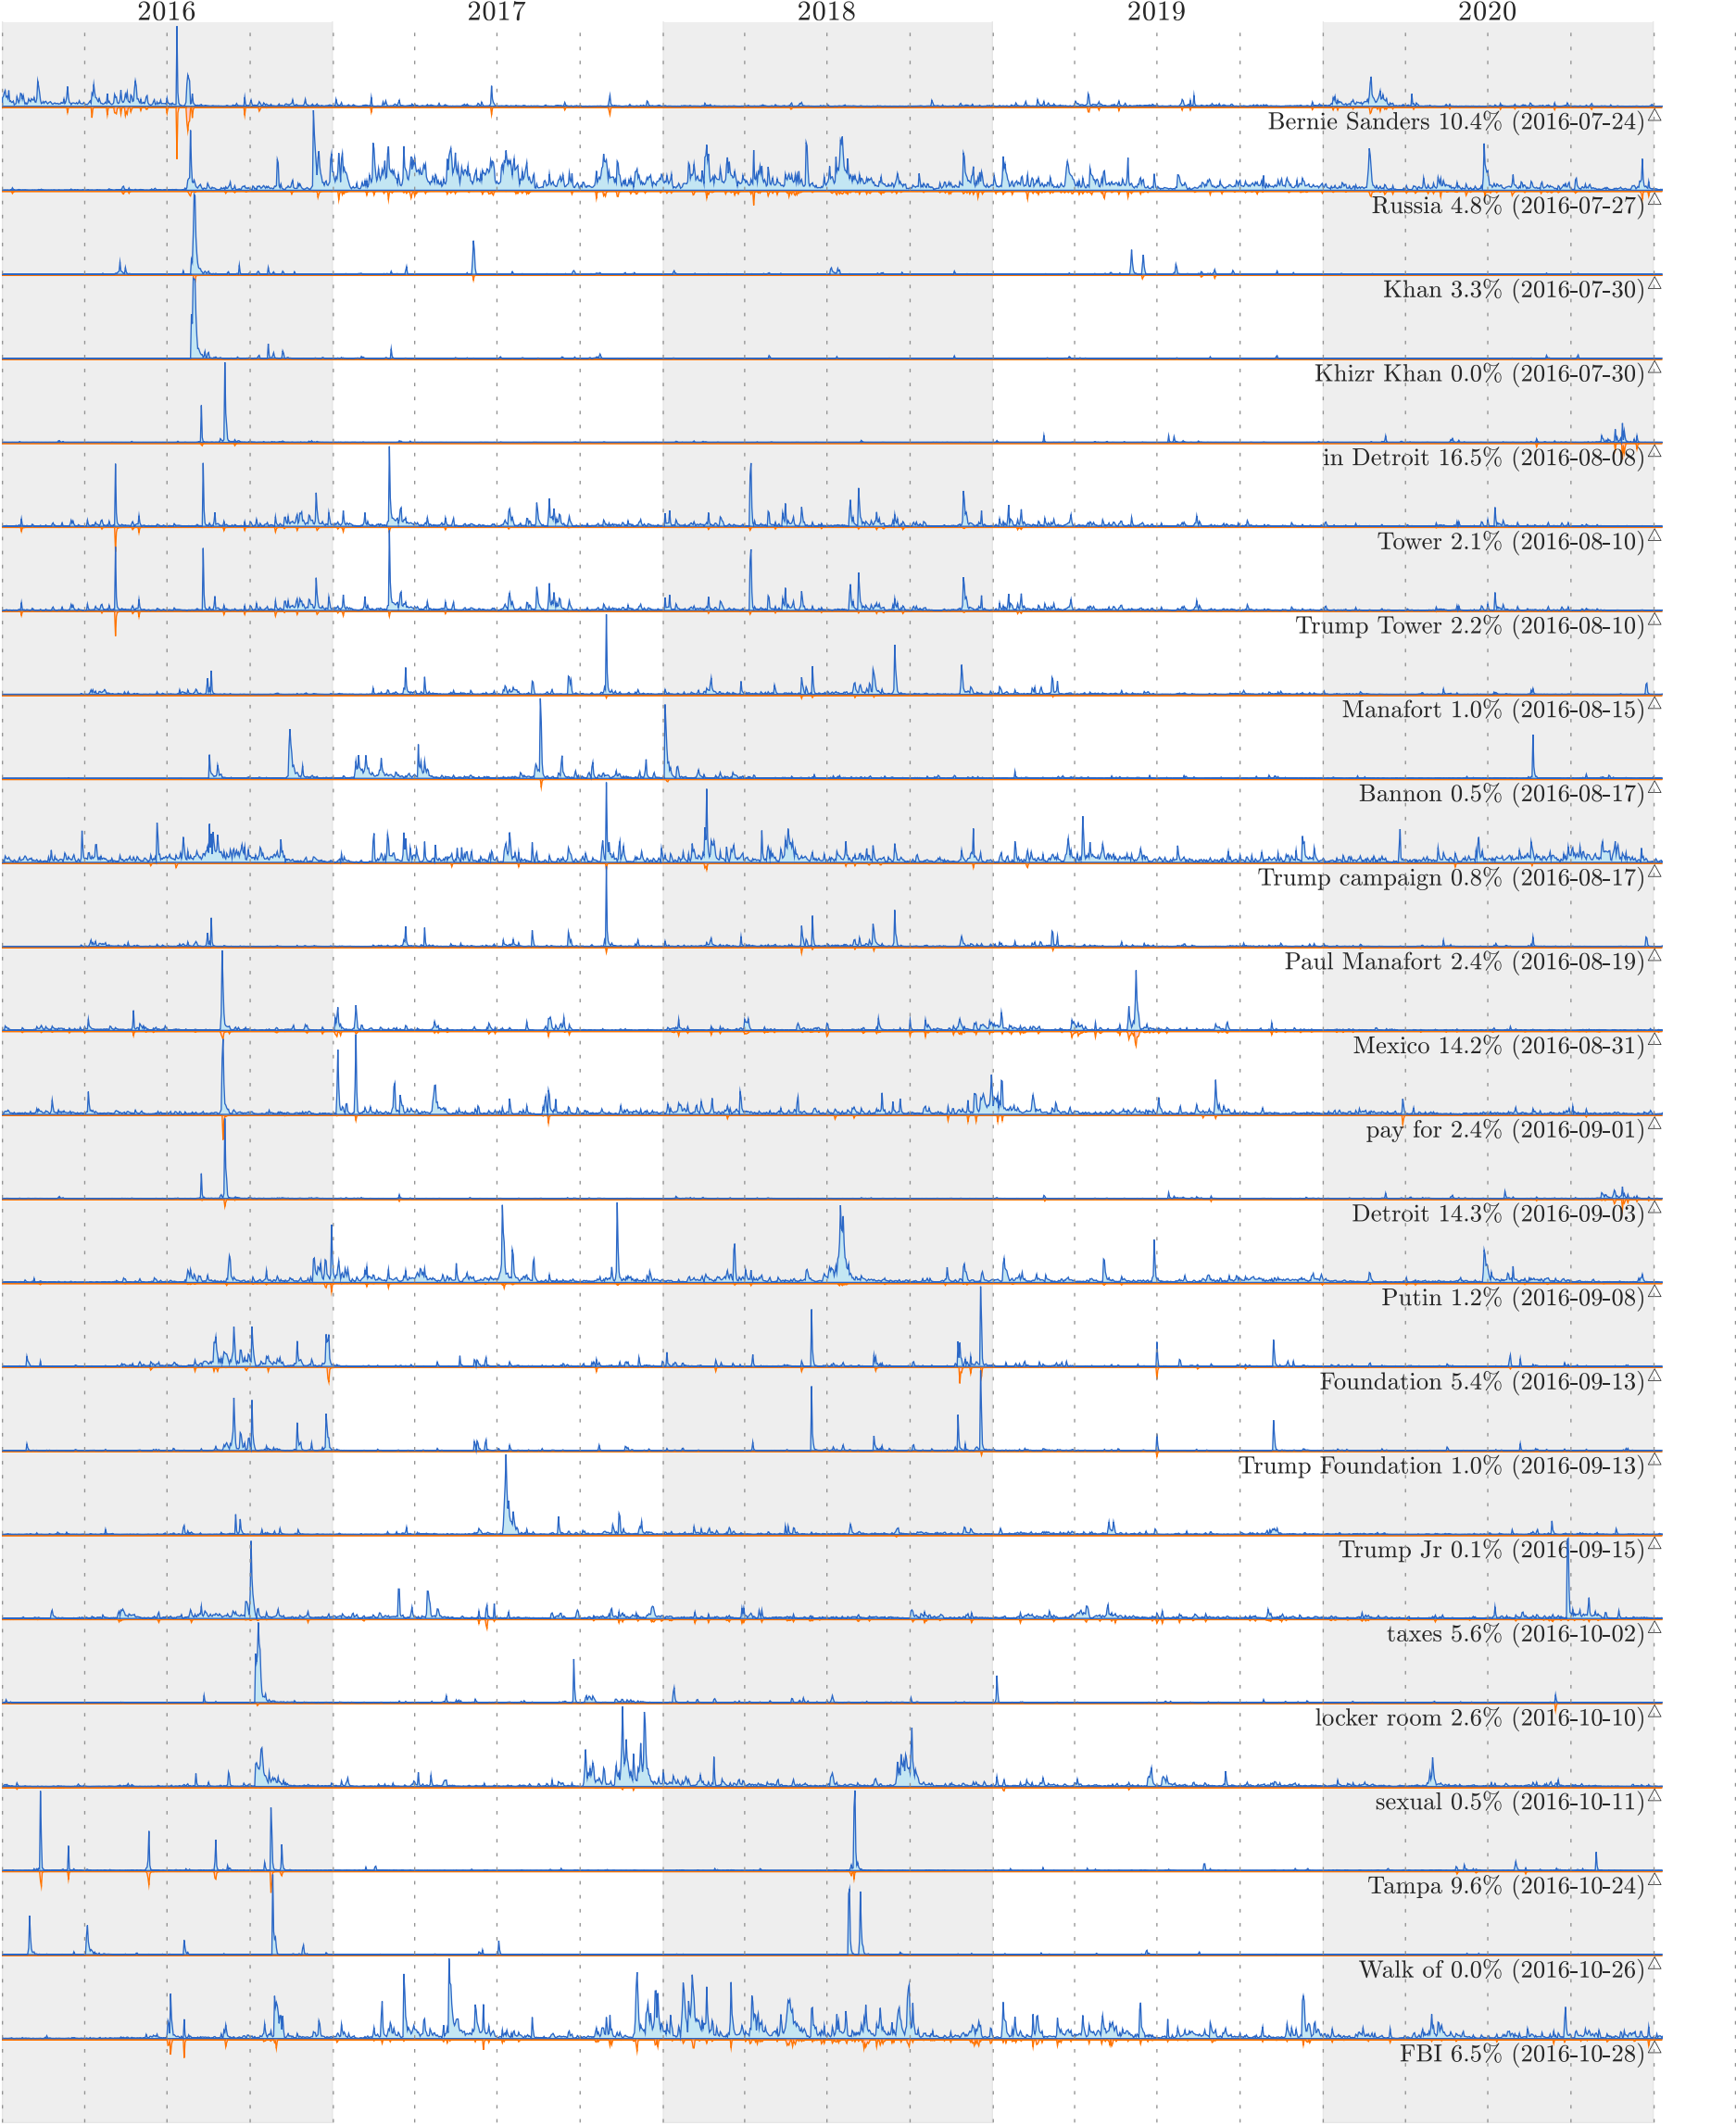

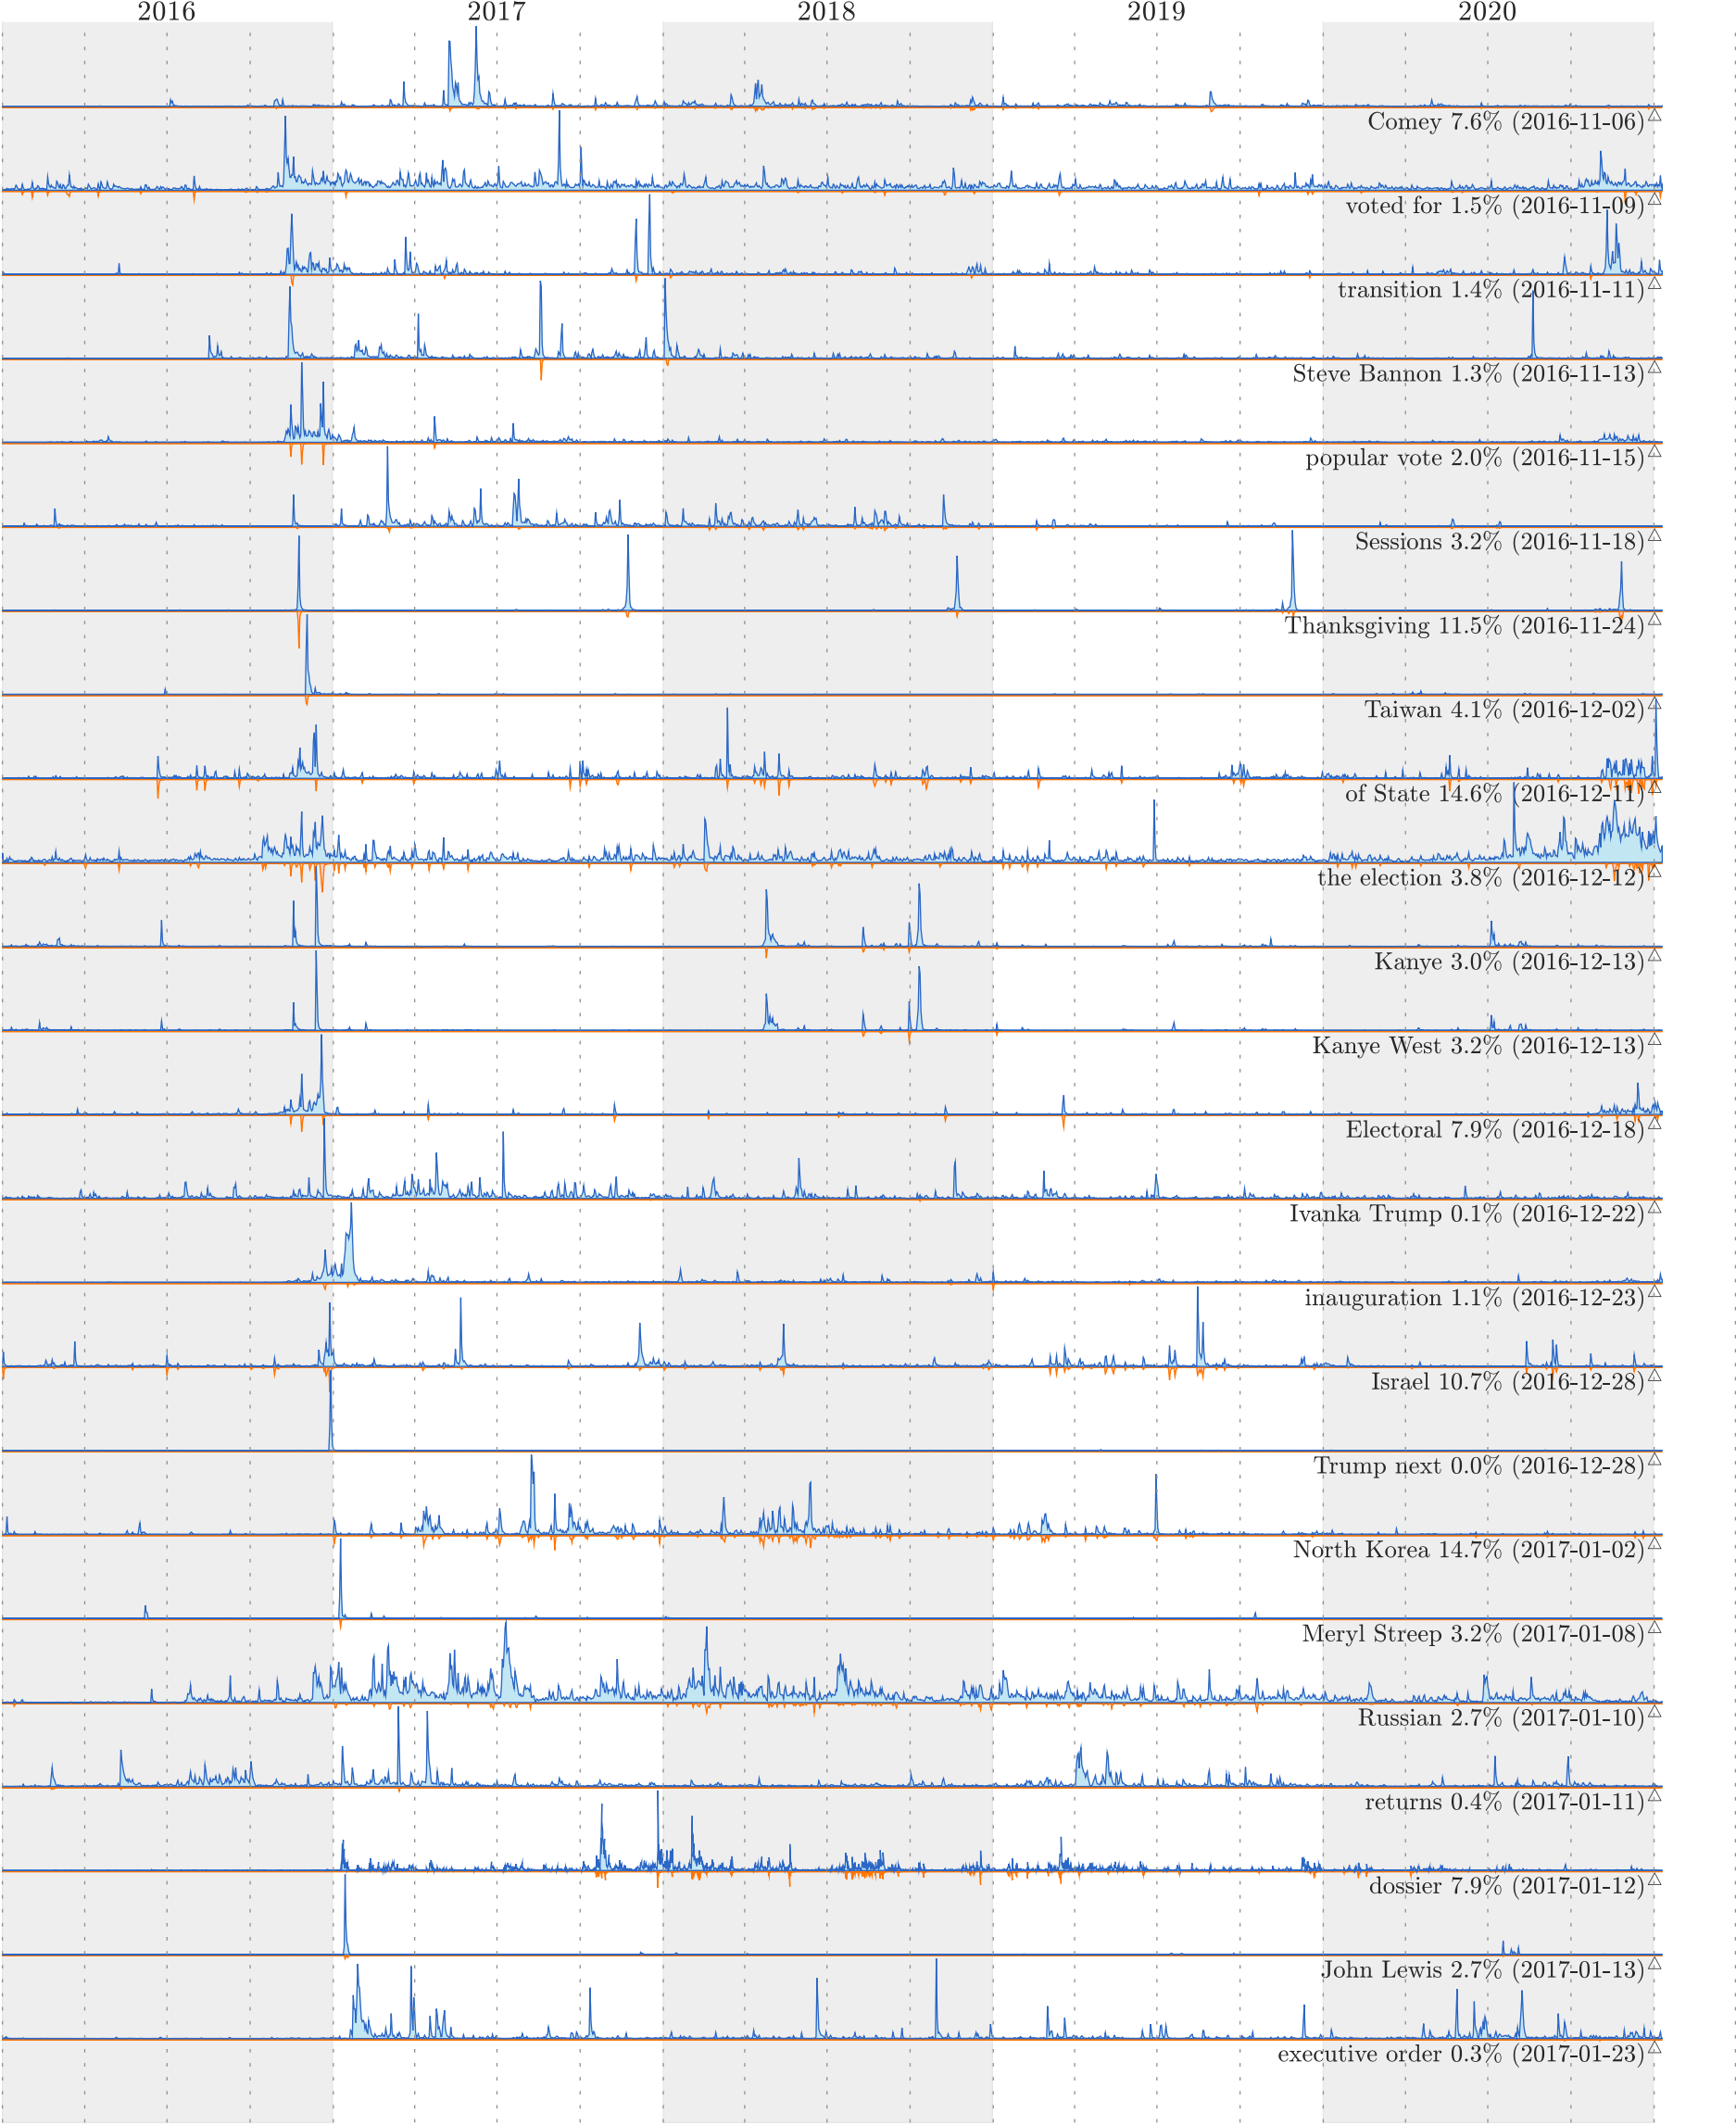



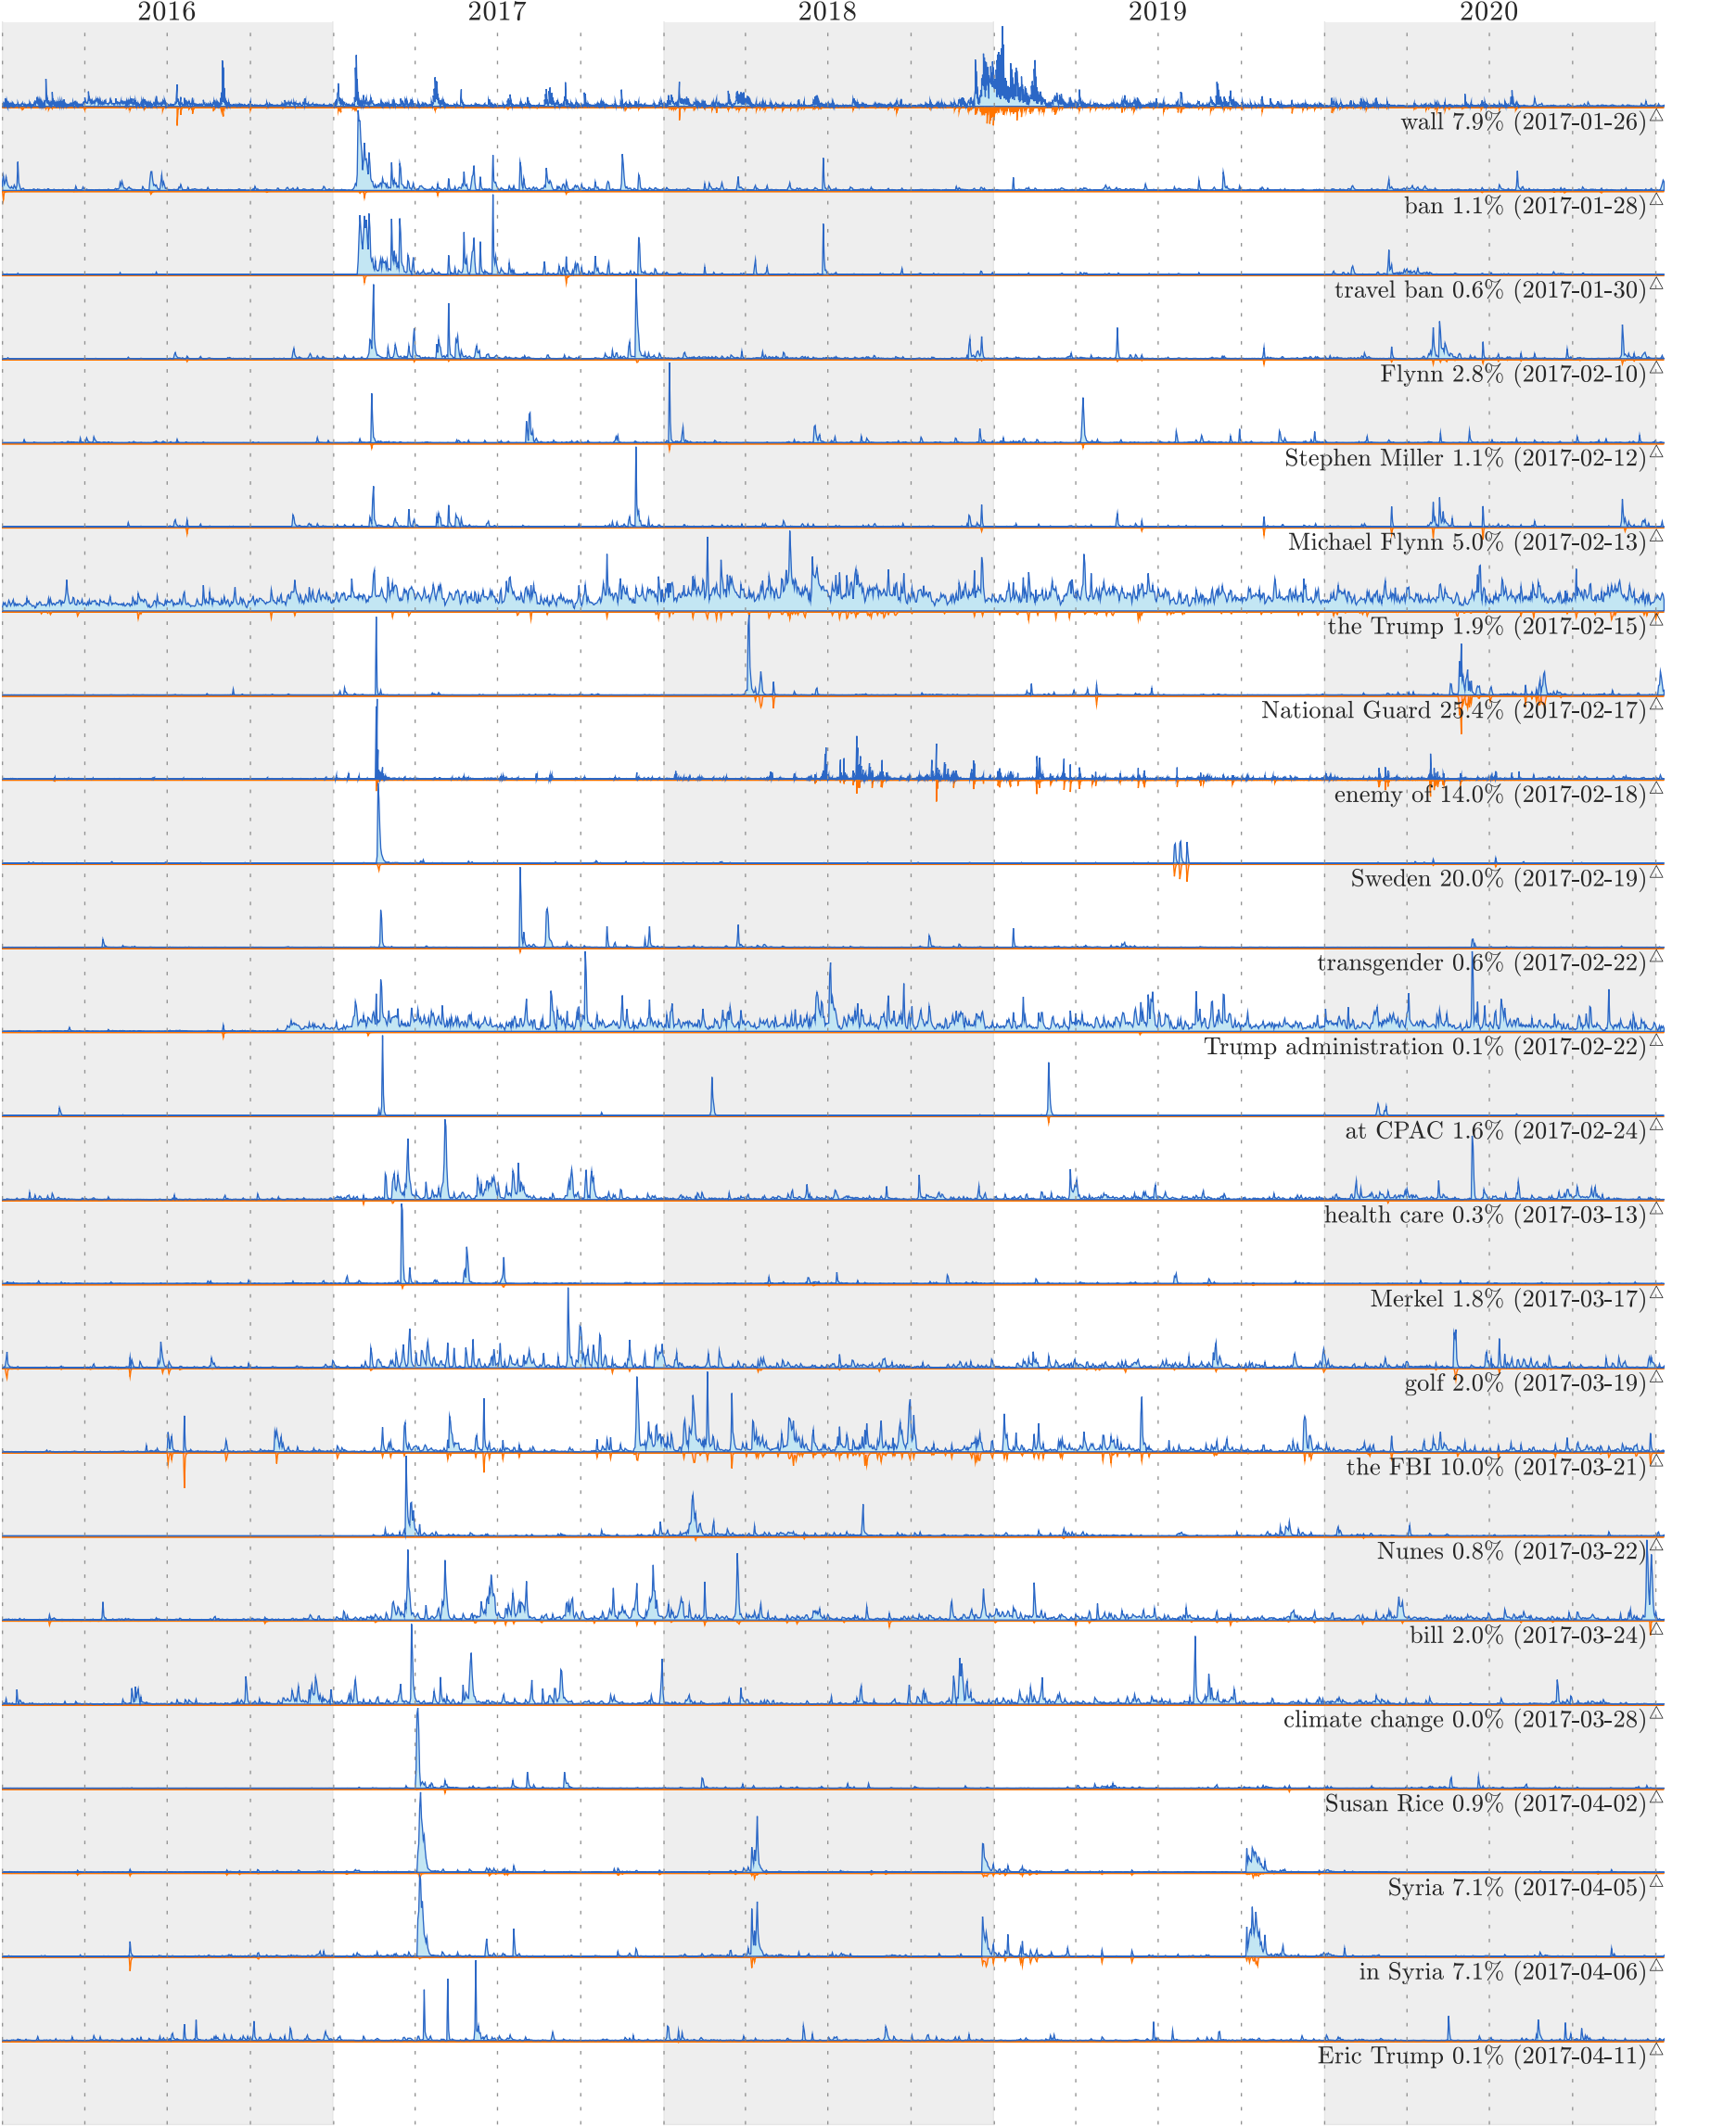

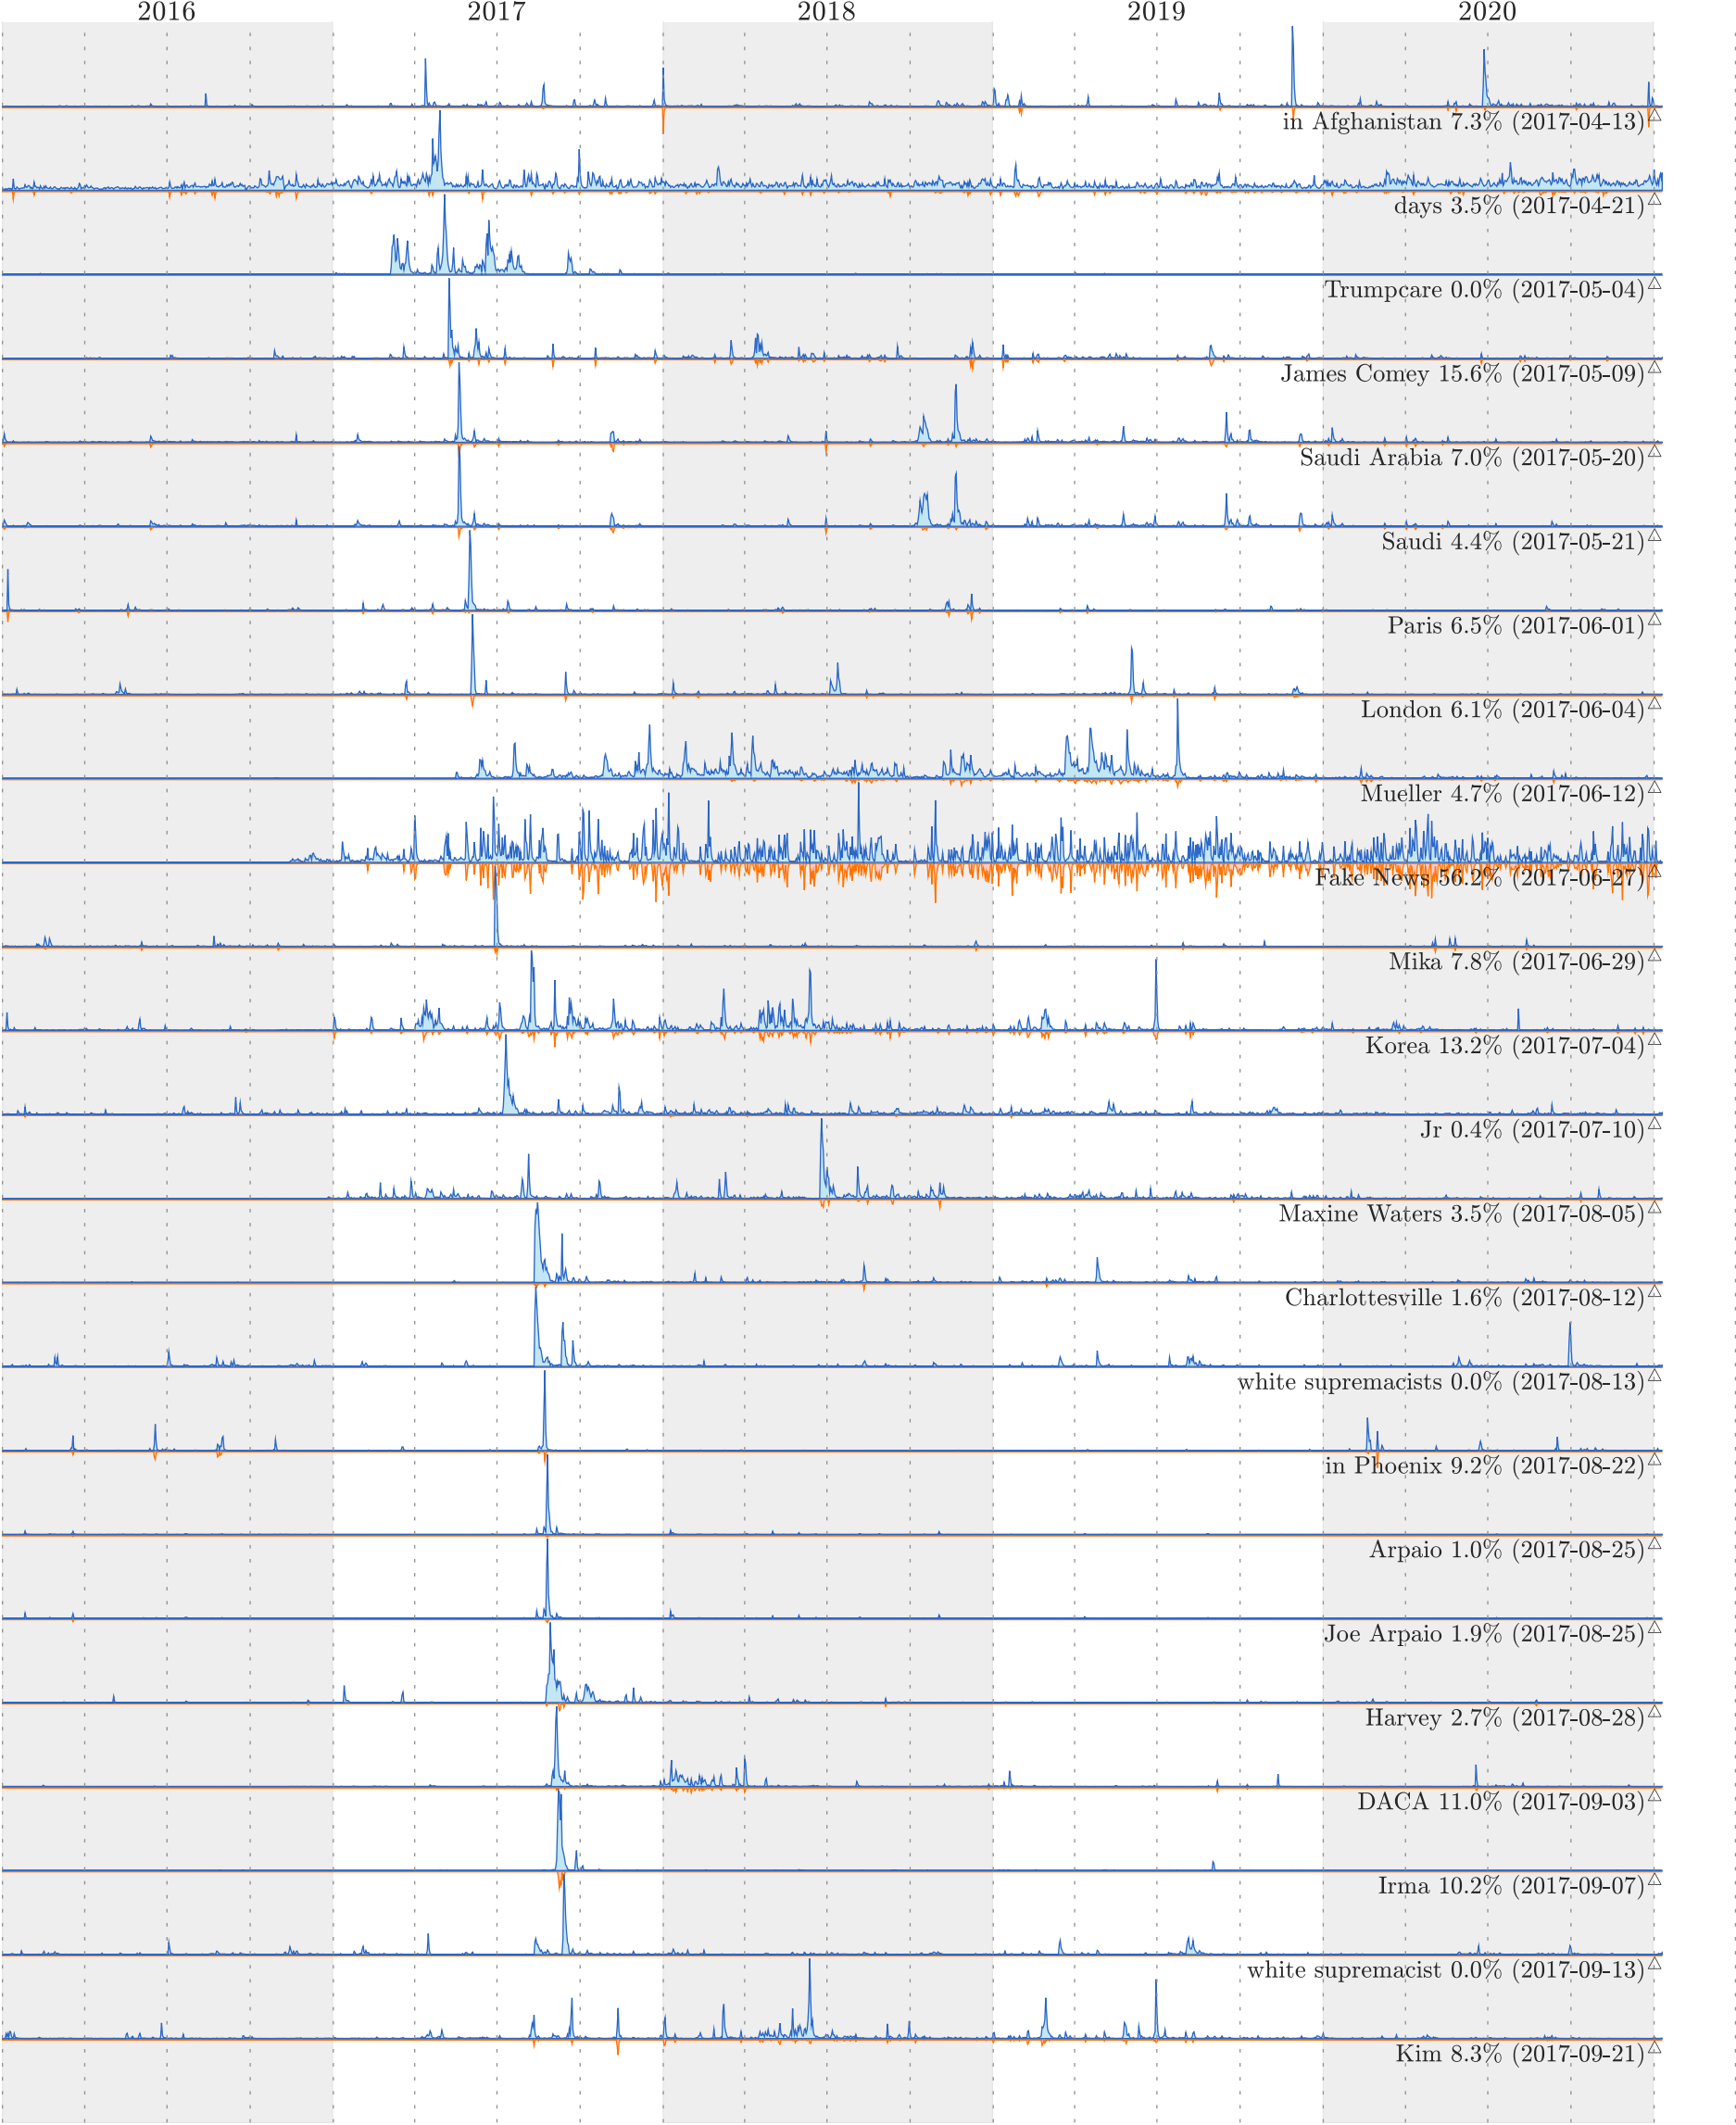

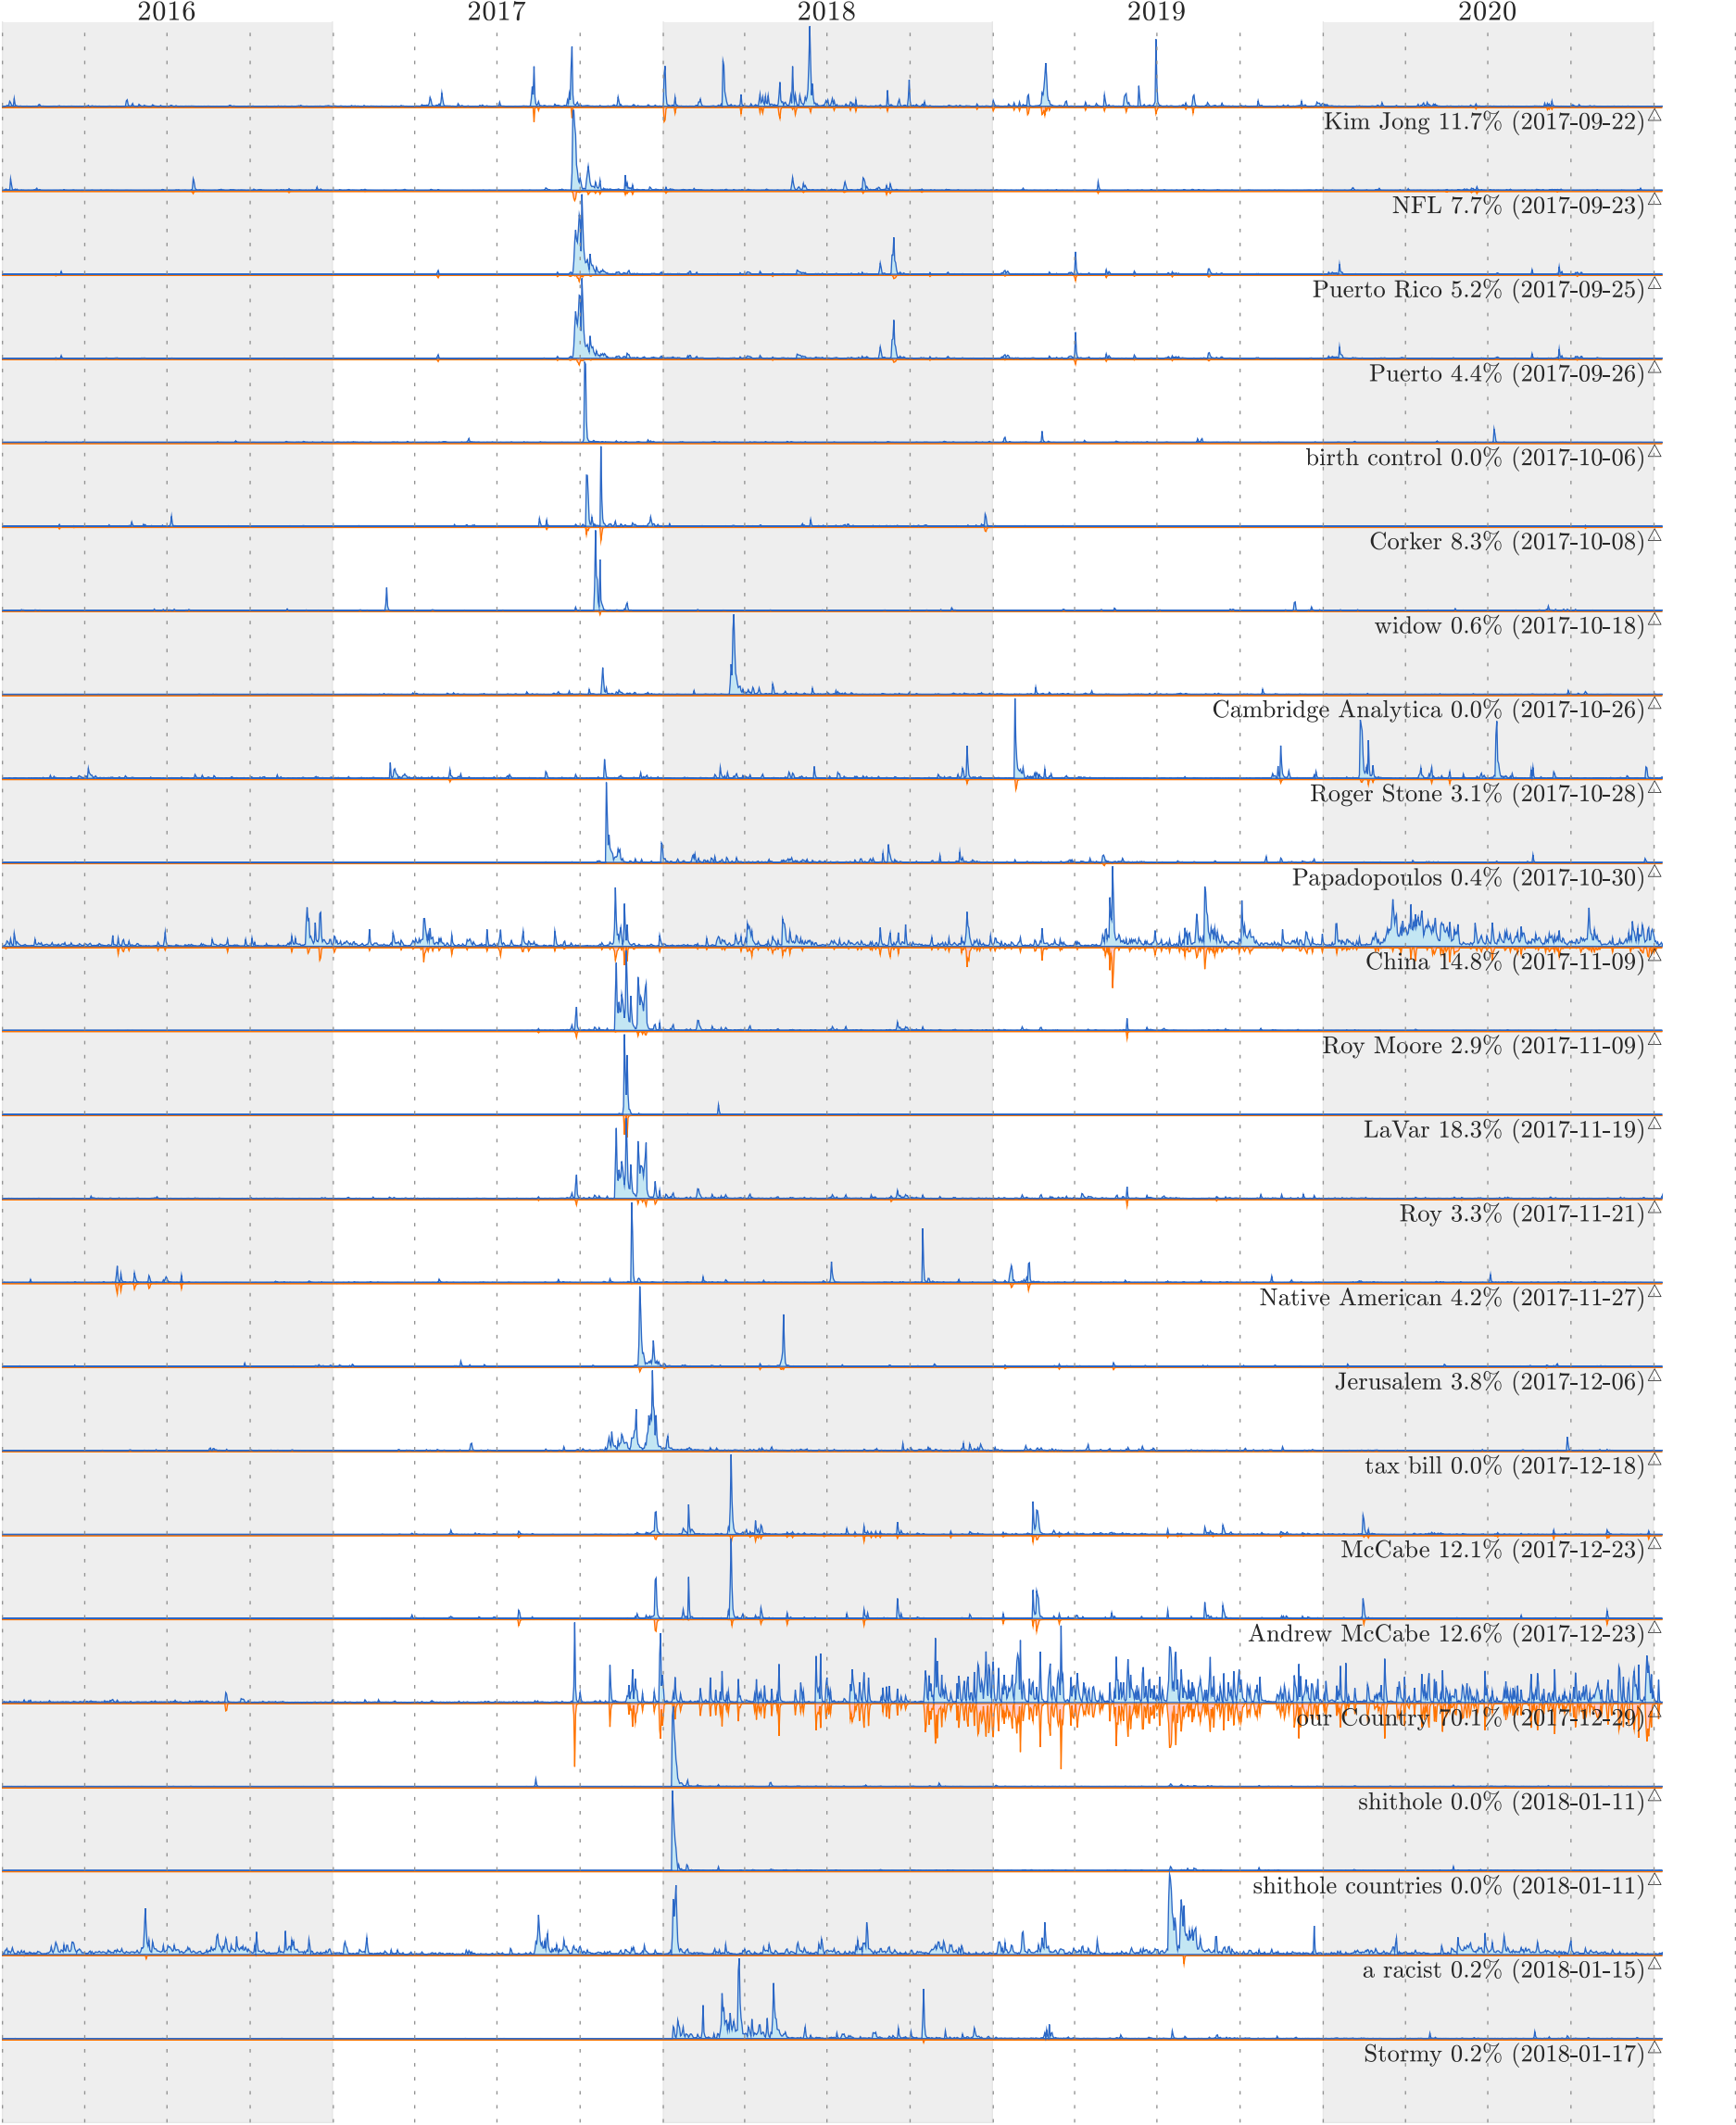

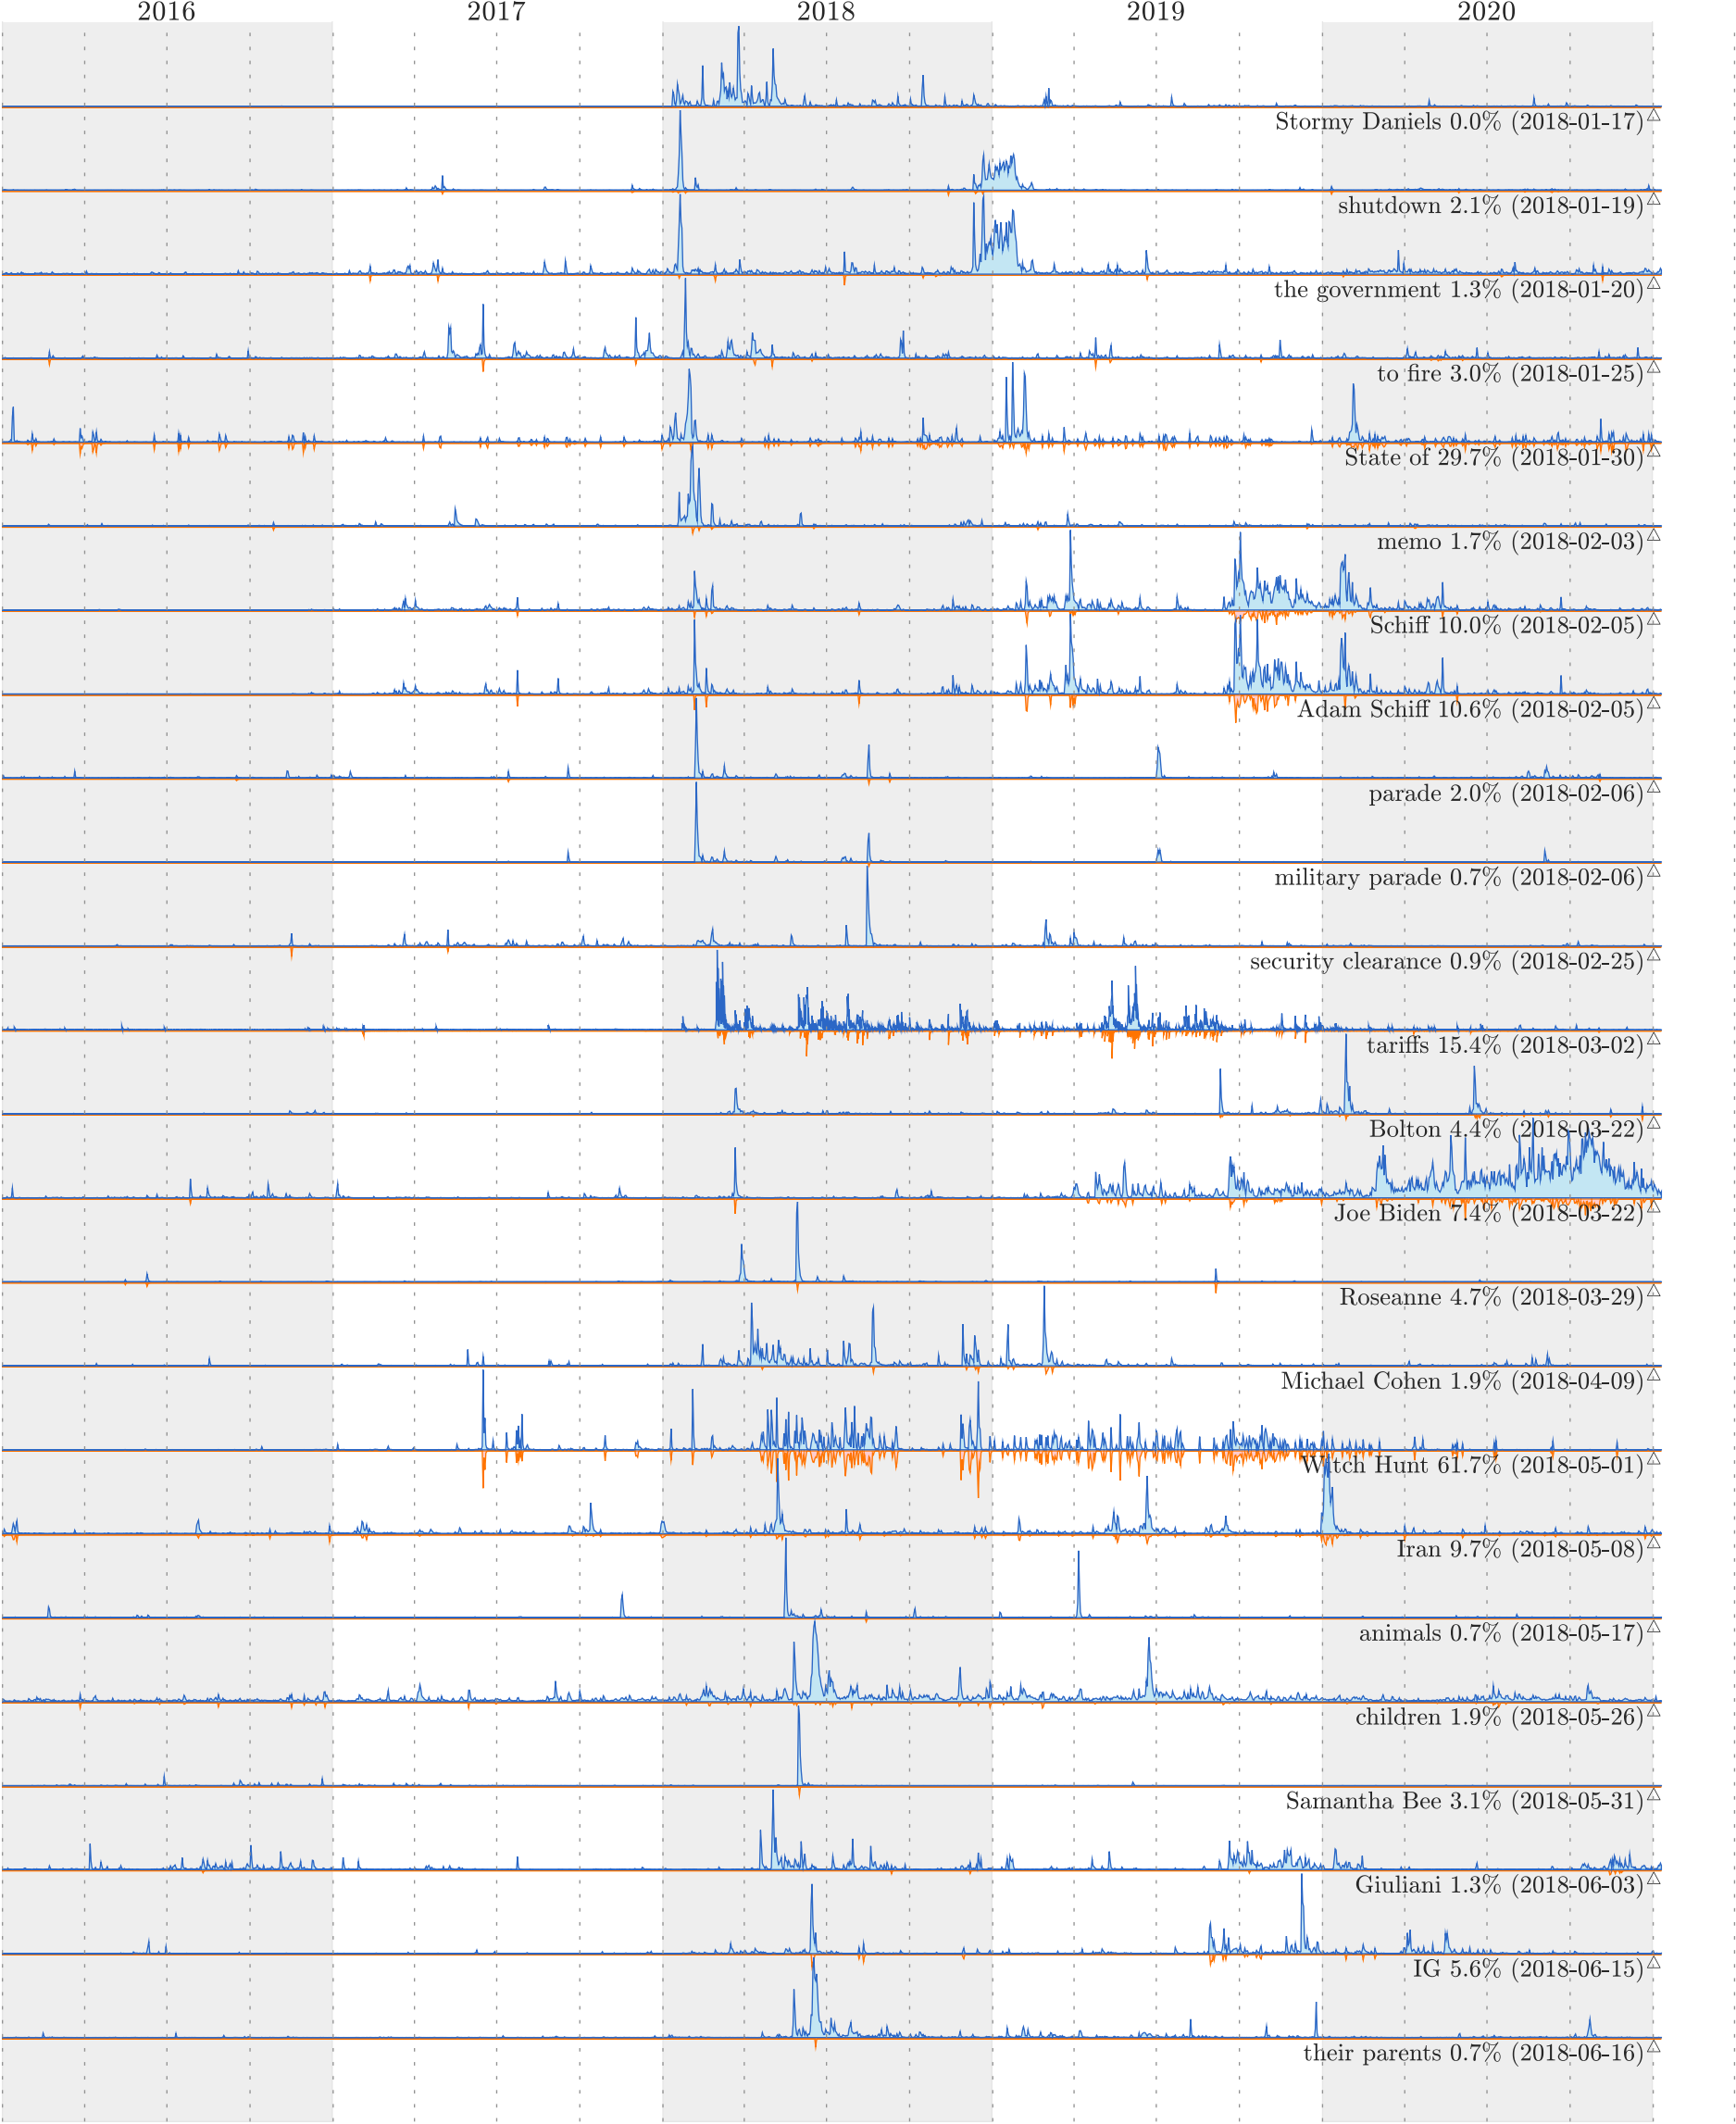



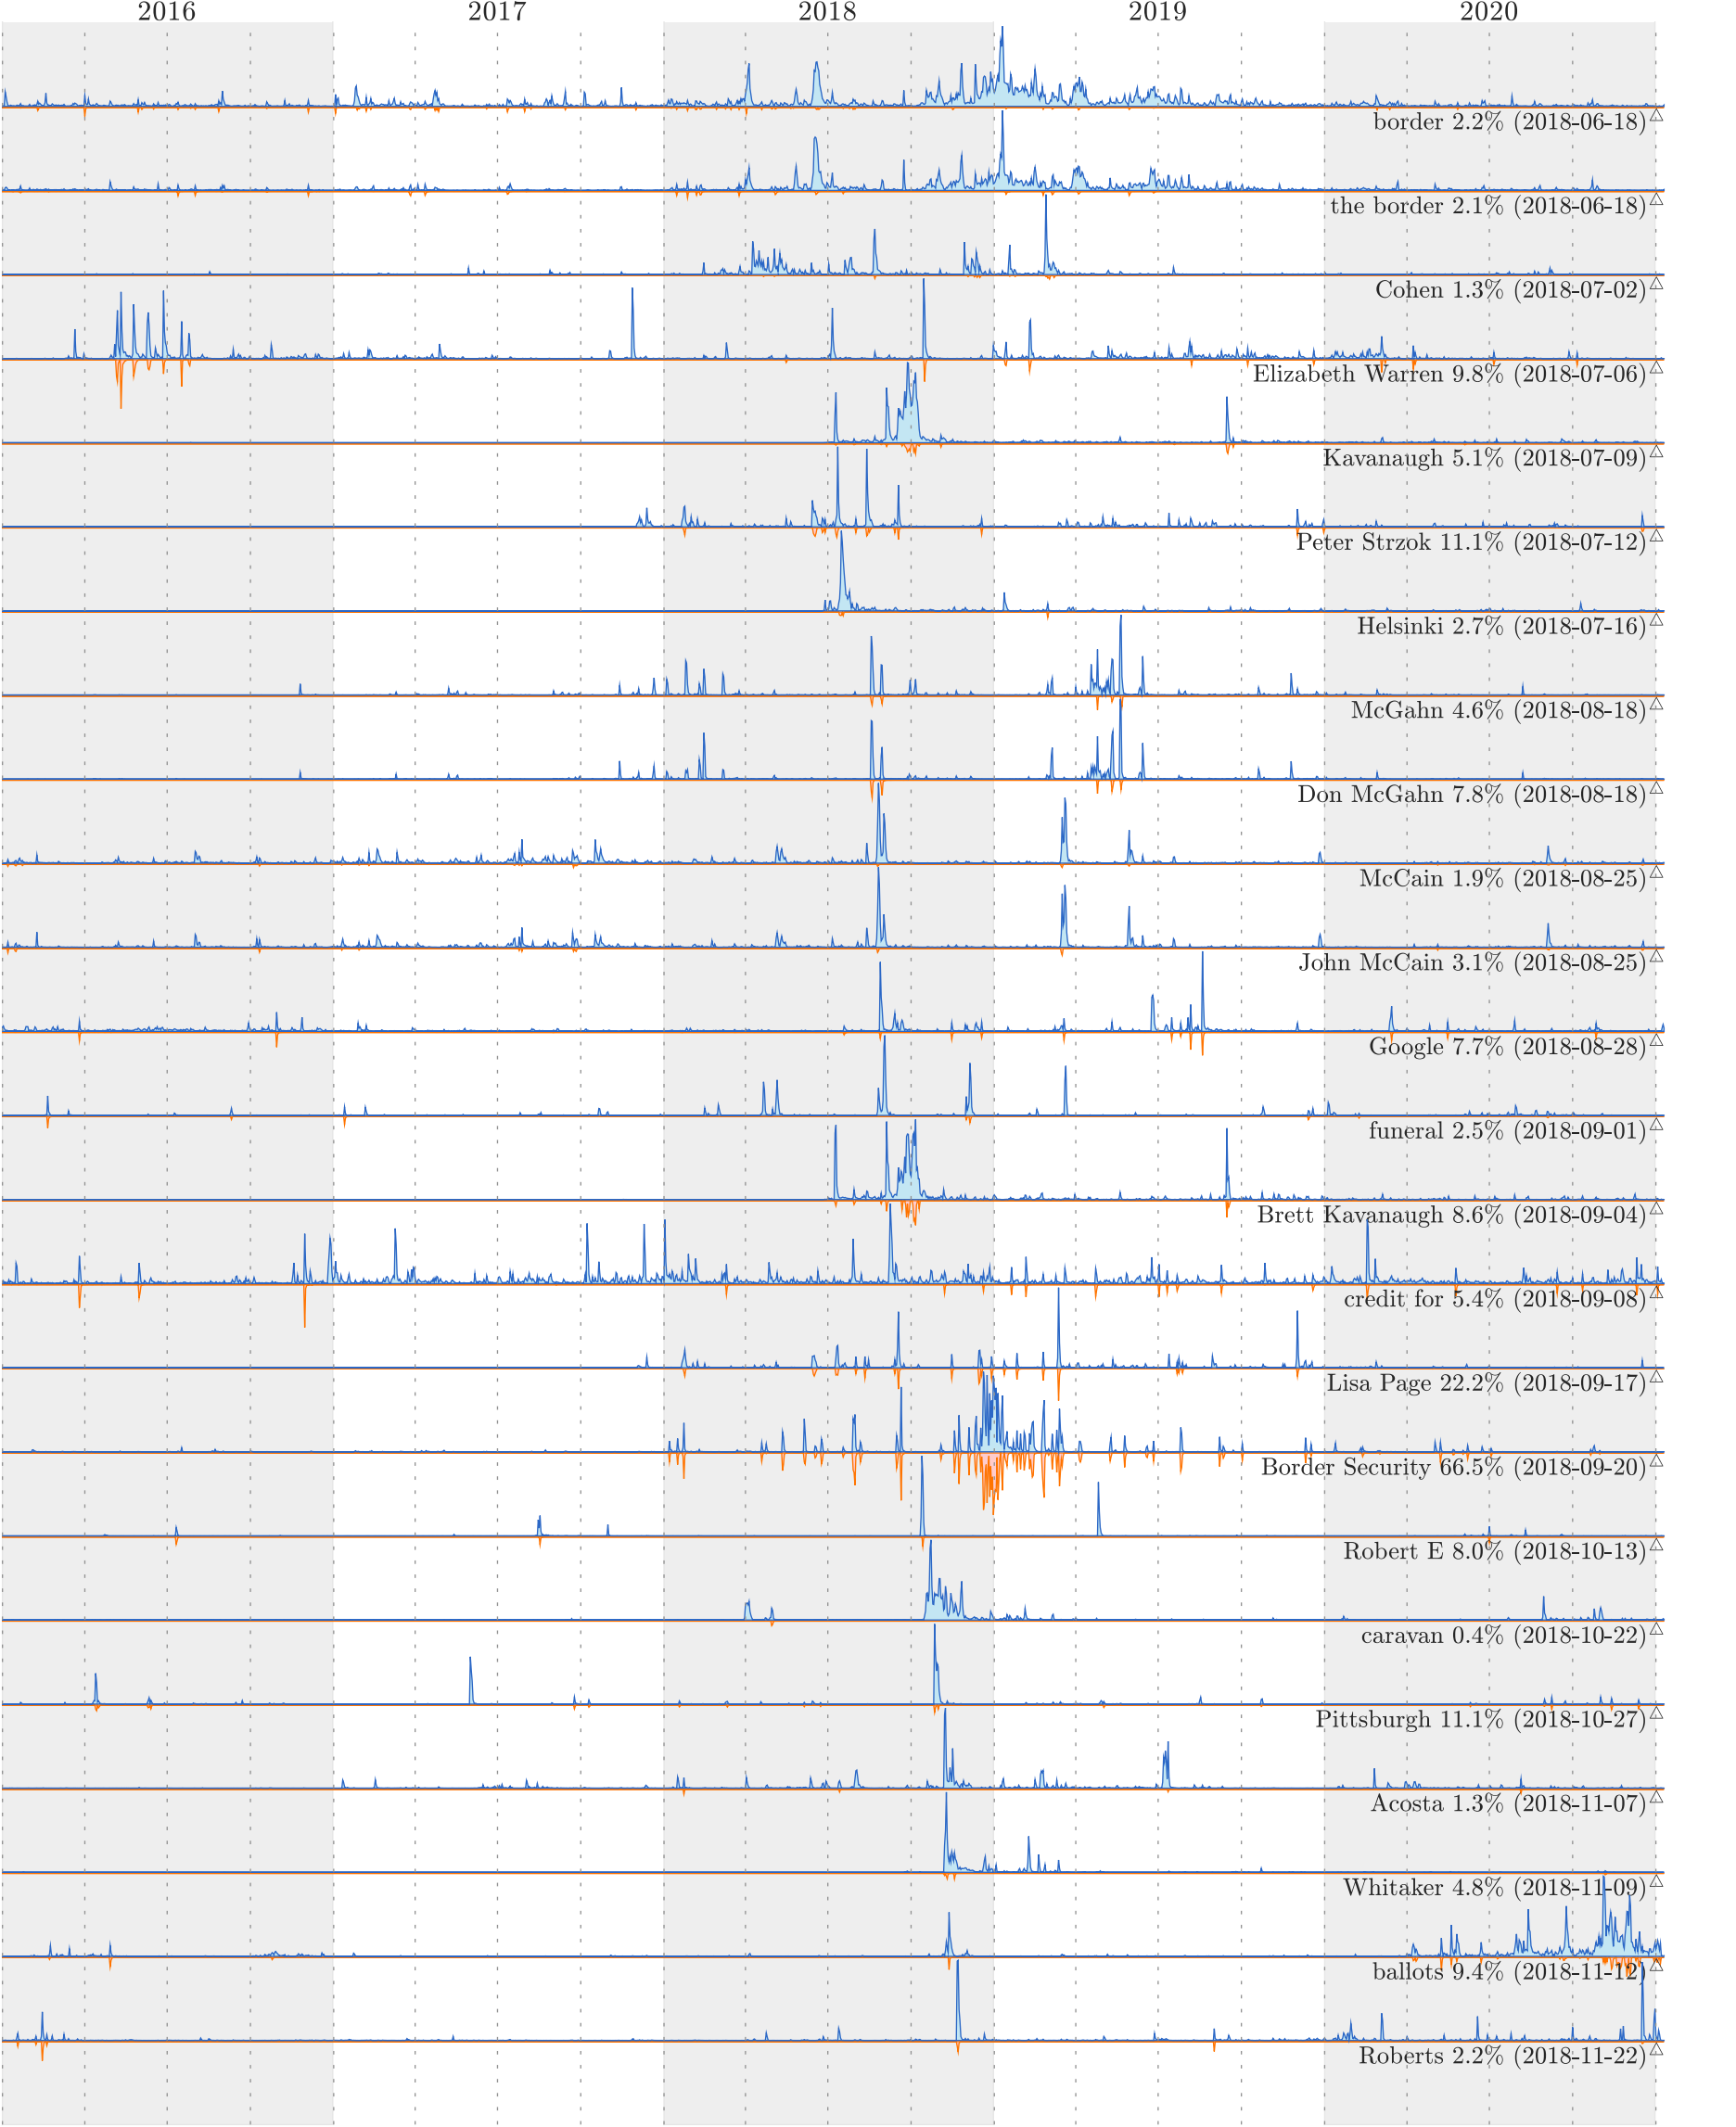

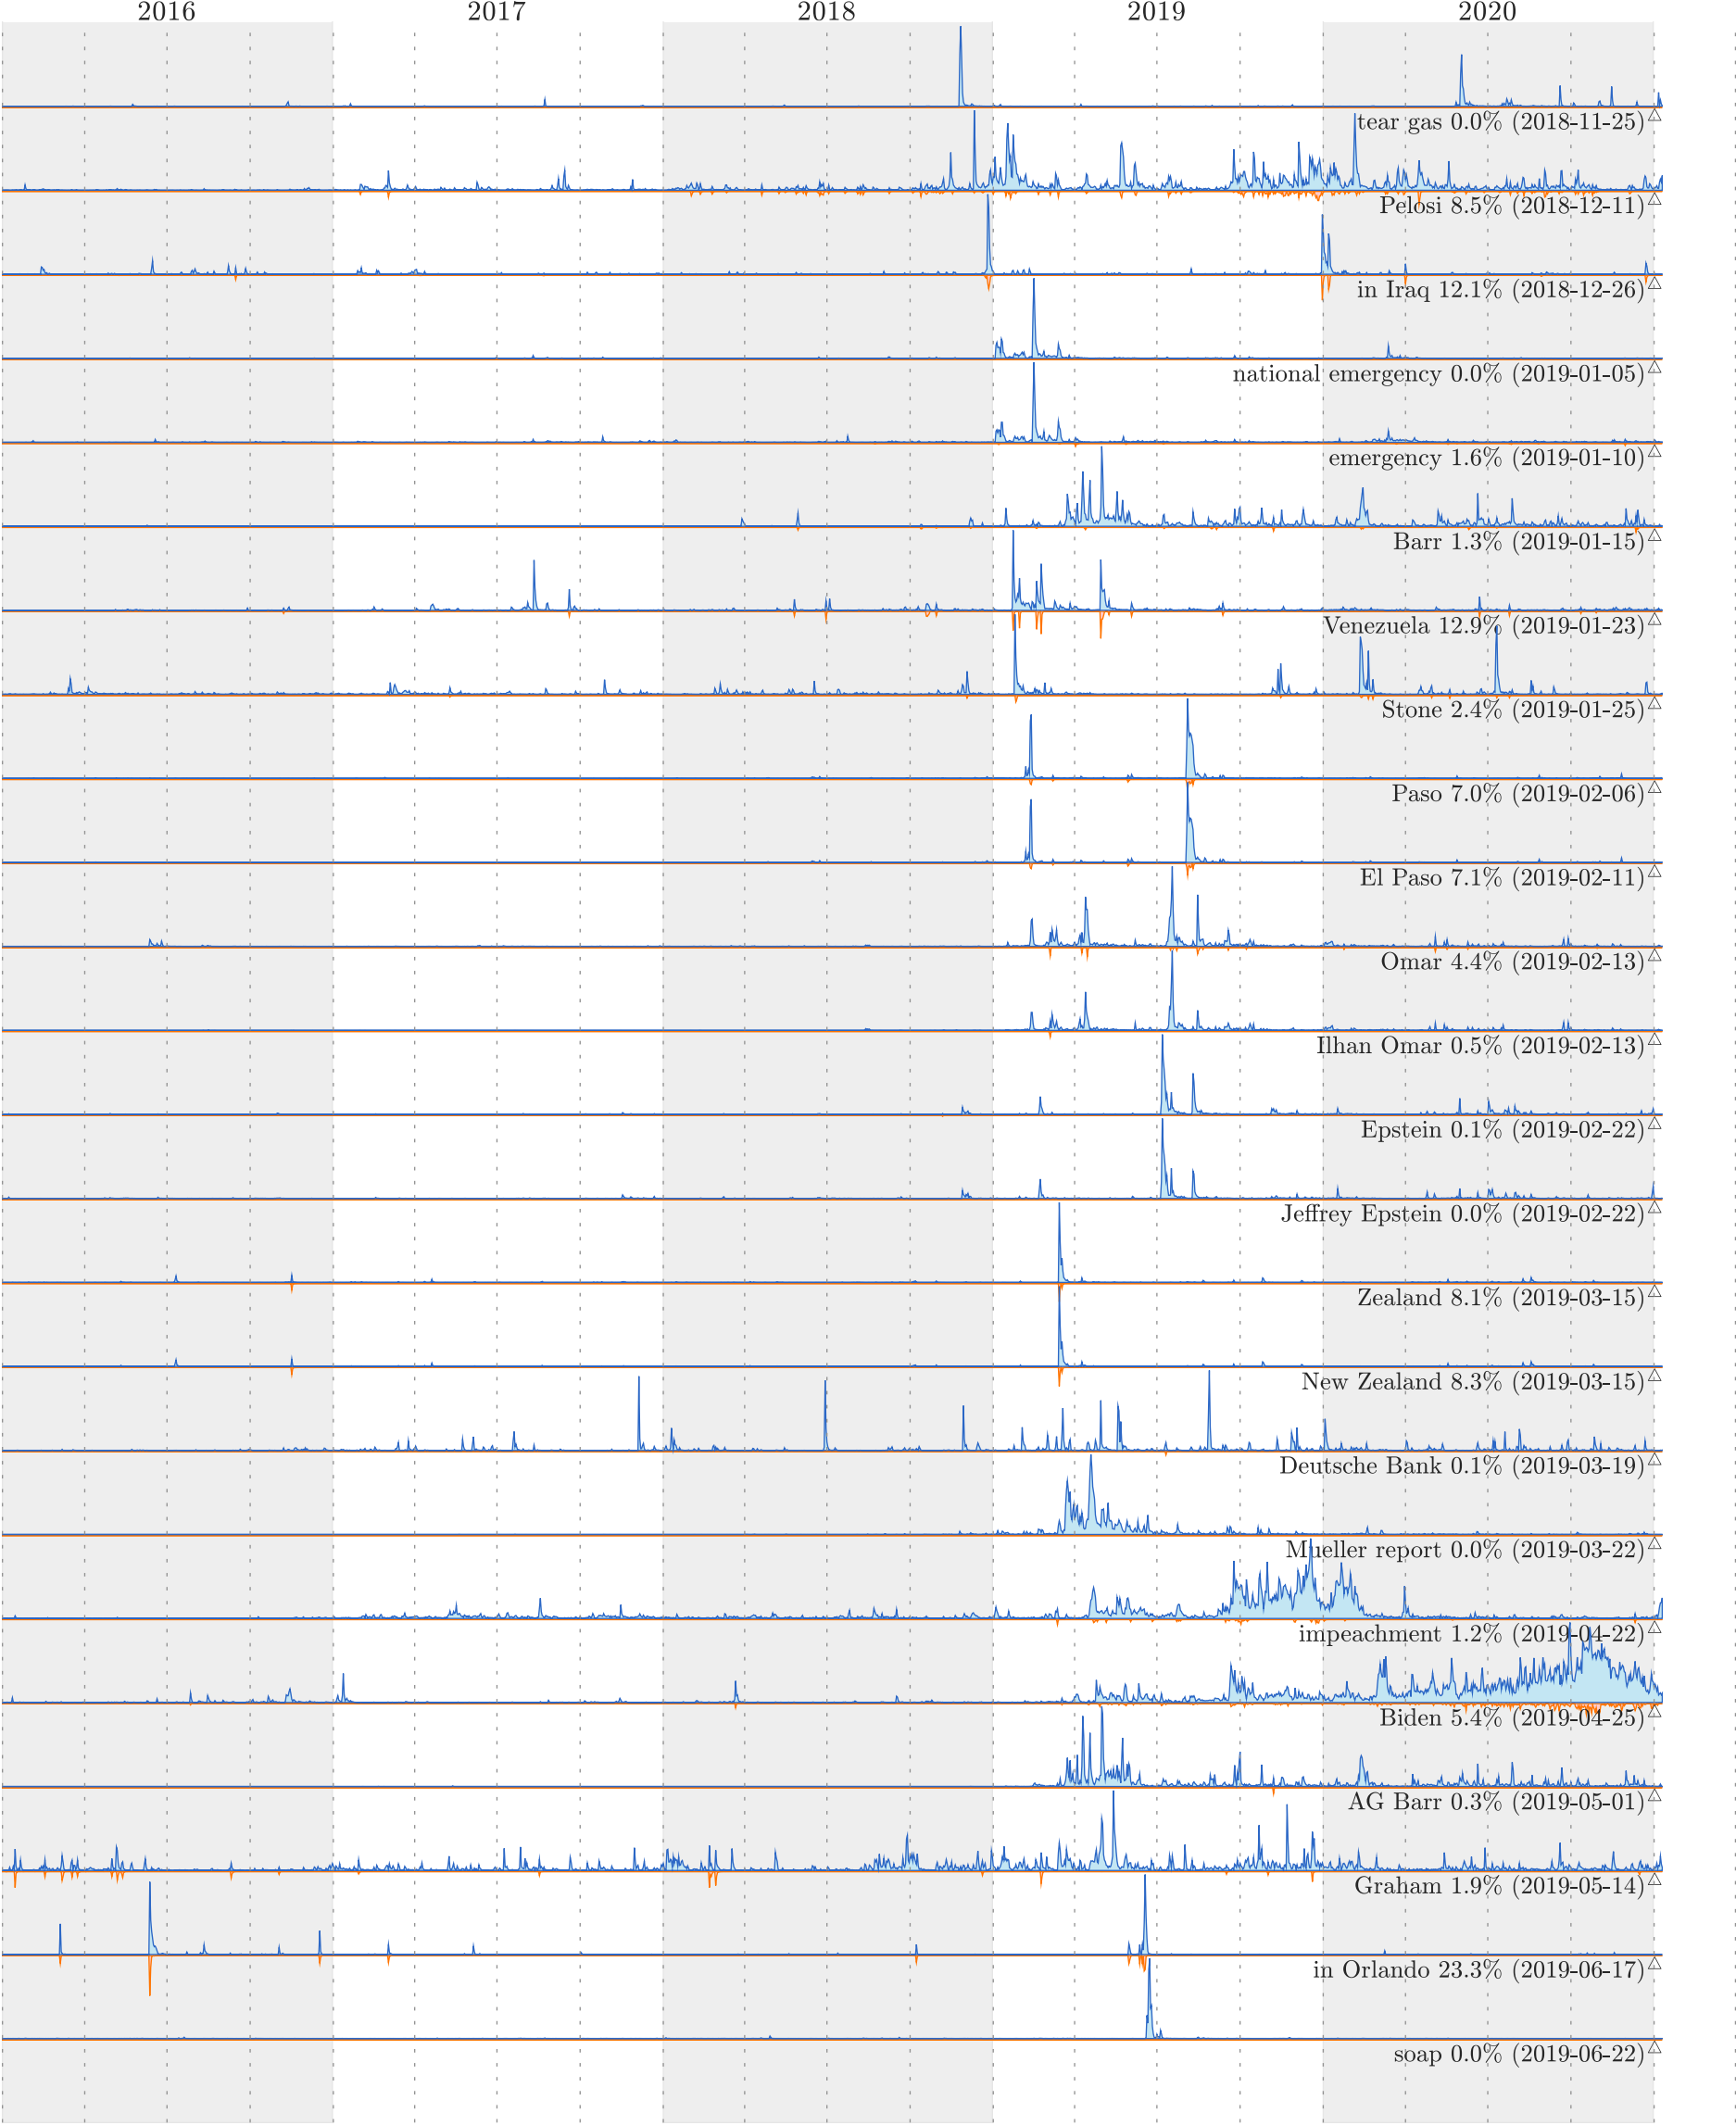

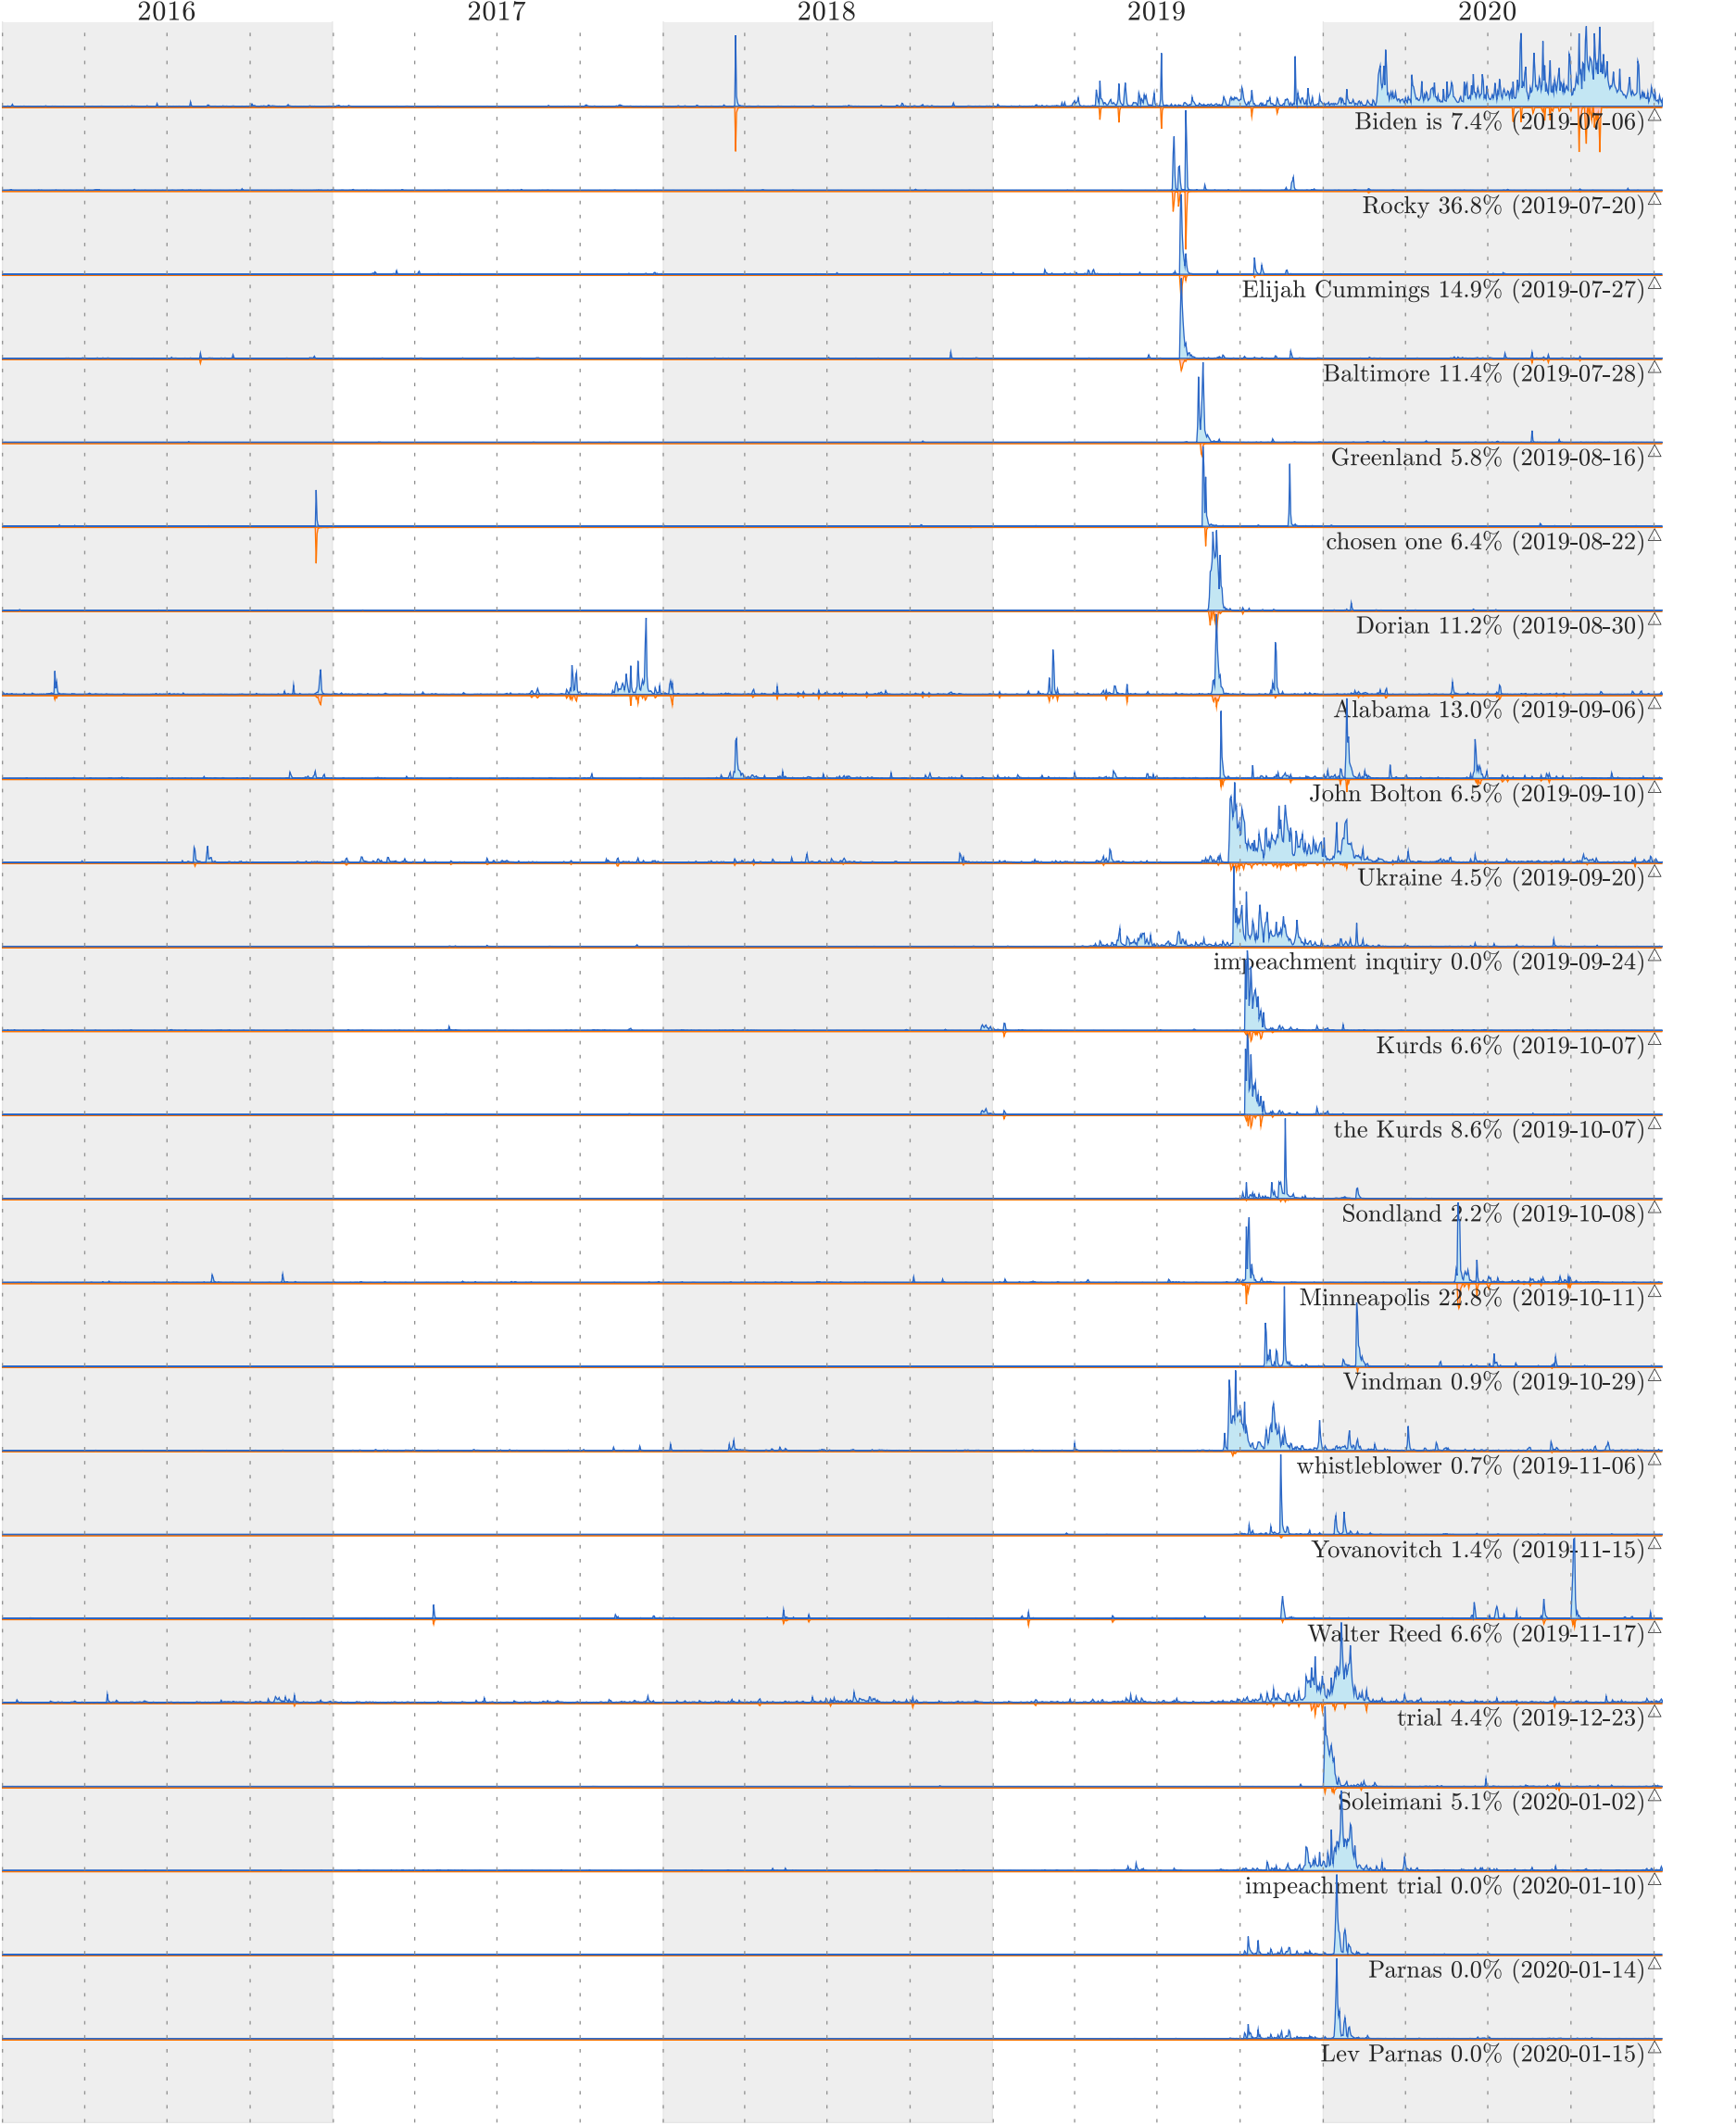

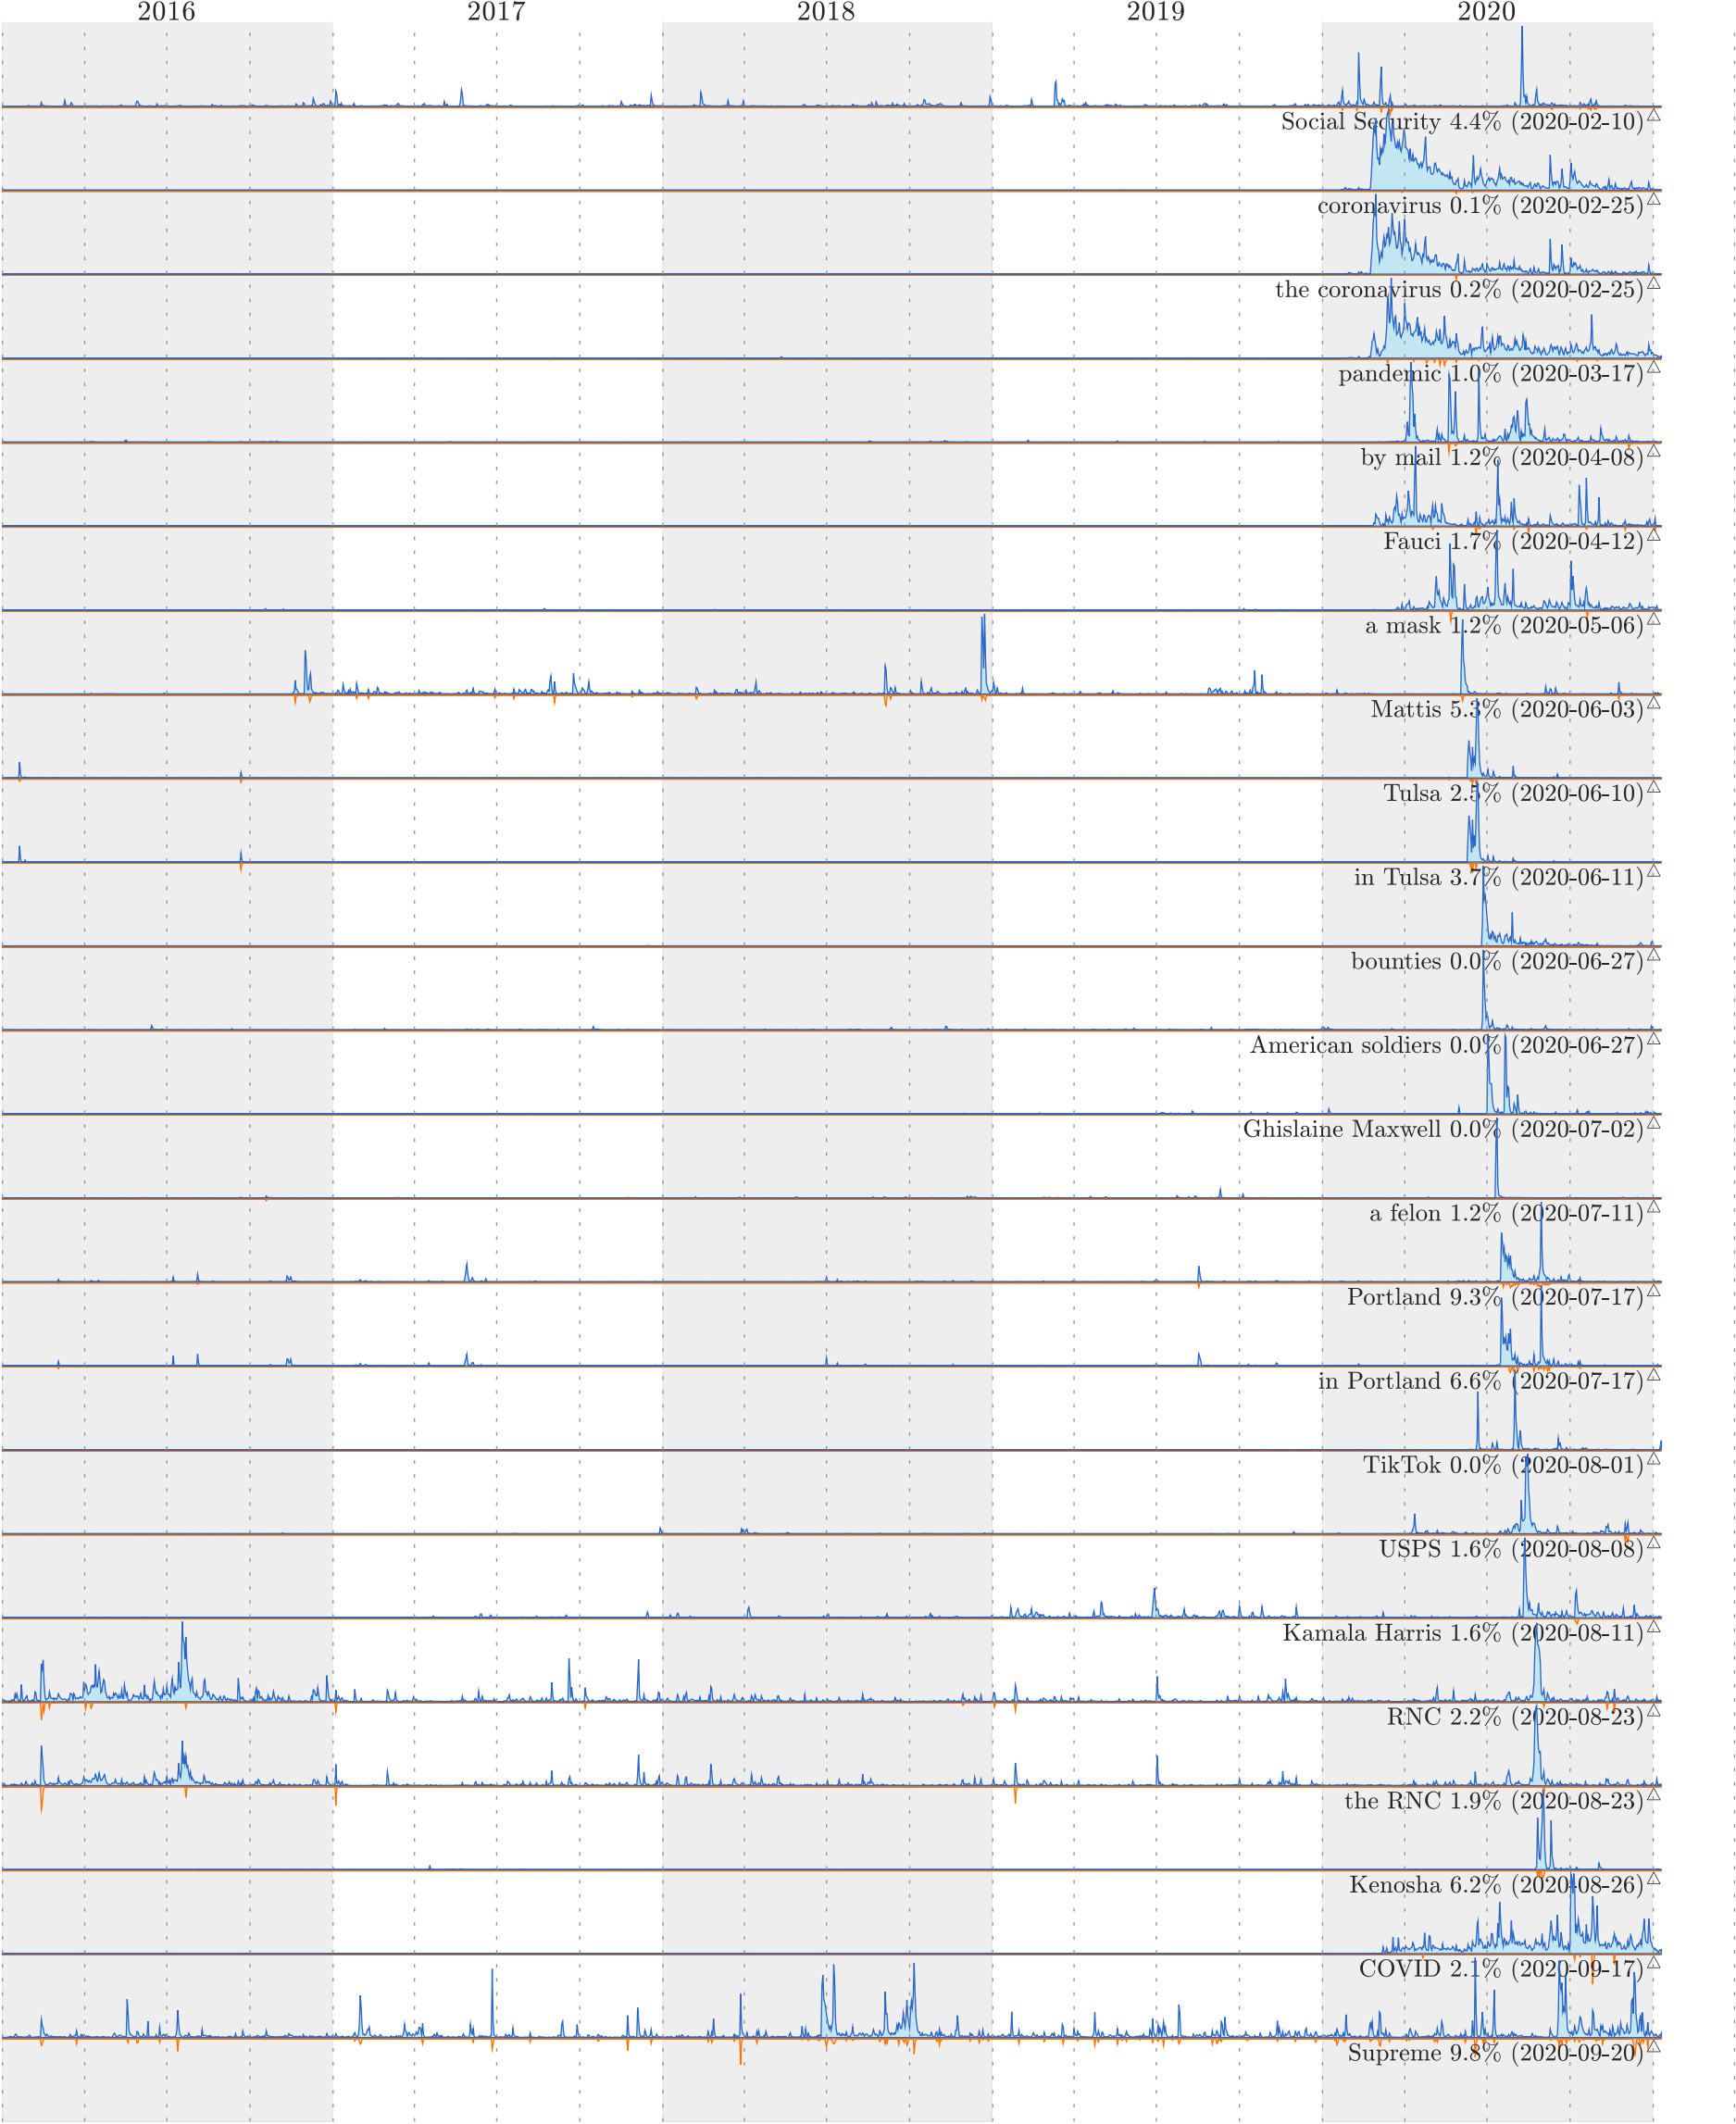



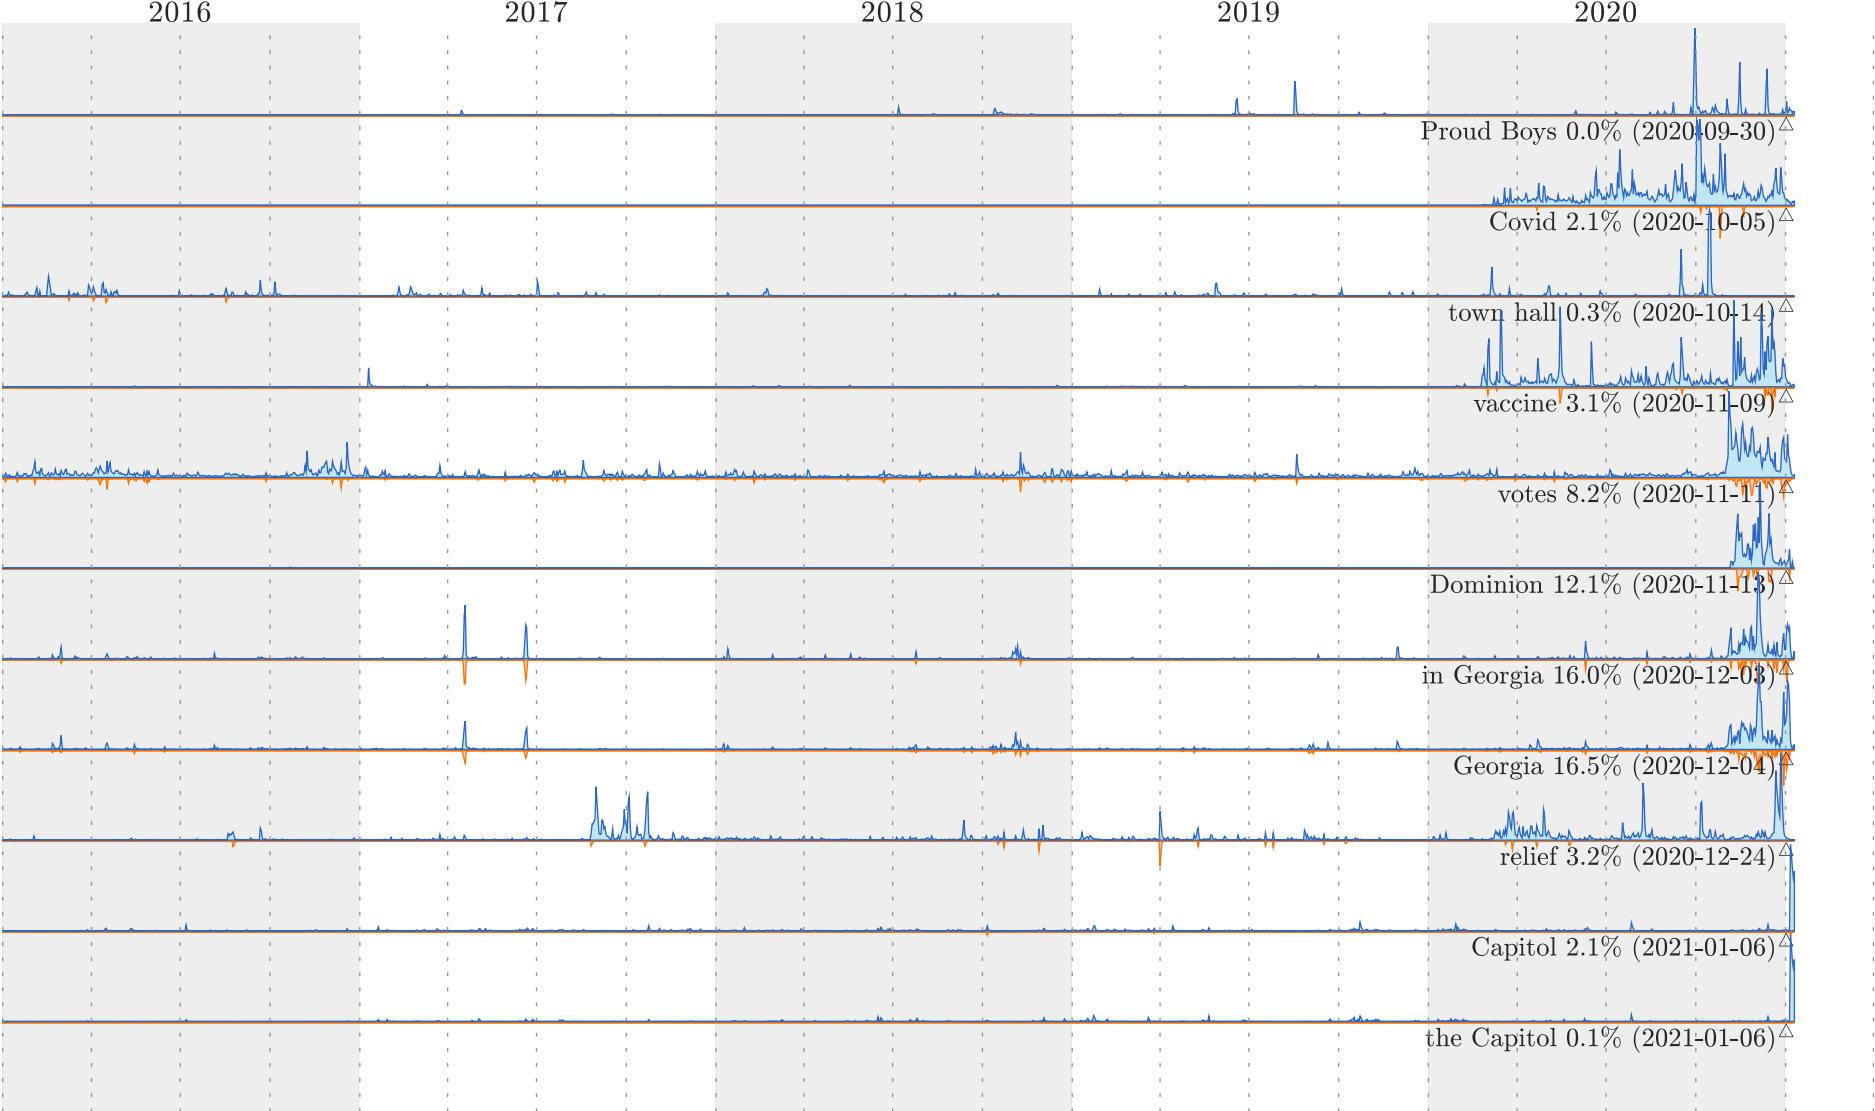

Supplement: Supplementary file 1 [file flipbook01_trump_major_storylines.pdf]
